# Supplementary material for: Sideband-resolved resonator electromechanics on the single-photon level based on a nonlinear Josephson inductance
Source: arXiv:1912.08731 ancillary file (2019-12-18)
Supplement: Supplementary file 1 [file SI.pdf]

# Sideband-resolved resonator electromechanics on the single-photon level based on a nonlinear Josephson inductance

Philip Schmidt,[1,2] Mohammad T. Amawi,[1,2] Stefan Pogorzalek,[1,2] Frank Deppe,[1,2,3] Achim Marx,[1] Rudolf Gross,[1,2,3] and Hans Huebl[1,2,3,*]

[1] *Walther-Meißner-Institut, Bayerische Akademie der Wissenschaften, Walther-Meißner-Str. 8, 85748 Garching, Germany*

[2] *Physik-Departement, Technische Universität München, James-Franck-Str. 1, 85748 Garching, Germany*

[3] *Munich Center for Quantum Science and Technology (MCQST), Schellingstr. 4, D-80799 München*

(Dated: December 18, 2019)

* huebl@wmi.badw.de

# I. SAMPLE AND SETUP

## A. Sample fabrication

Fabrication starts with a commercial high resistivity silicon wafer ($> 10\,\mathrm{k\Omega cm}$) diced in $10 \times 6\,\mathrm{mm}^2$ chips. After cleaning, we spin coat the substrate with a double layer resist and define the pattern of the entire sample using electron beam lithography. This includes the coplanar waveguide representing the feedline, the coplanar waveguide (CPW) being part of the microwave resonator, as well as the direct-current superconducting quantum interference device (dc-SQUID). The latter includes the Josephson junctions. After development, we deposit two layers of aluminium with thicknesses of 40 nm and 70 nm using electron beam evaporation in a shadow-angle evaporation configuration. Between the two evaporation steps, we include an oxidation step. After a lift-off process, the sample is annealed at $350^\circ$ C in atmosphere for 30 minutes, to mechanically relax the structure and enhance the tensile stress of the nanostrings. To freely suspend the doubly-clamped nanostrings, we then perform a two step reactive ion etching process on the entire chip: (i) we initially etch directionally into the silicon and then (ii) isotropically under-etch parts of the aluminium thin film. This process releases the nanostrings and makes them mechanically compliant.

## B. Microwave setup

Figure S1 shows the various microwave setup configurations used for the experiments presented in this work. Panel **a** shows the details of the cryogenic microwave wiring inside the fridge which is not altered between the various experiments. All microwave tones are sent to the input of the sample box via the "signal in" line. The total microwave attenuation $\Lambda_{\mathrm{tot}} = \Lambda_{\mathrm{att}}\Lambda_{\mathrm{c}}\Lambda_{\mathrm{rt}}$ of the input line consists of microwave attenuators which add up to $\Lambda_{\mathrm{att}} = -42\,\mathrm{dB}$ mounted at the various temperature stages (cf. Fig. S1**a**), as well as the attenuations $\Lambda_{\mathrm{rt}}$ and $\Lambda_{\mathrm{c}}$ of microwave cables and components at room temperature and cryogenic temperatures, respectively. The room temperature attenuation $\Lambda_{\mathrm{rt}}$ is calibrated for each microwave configuration (cf. Fig. S1**b**, **c**, while the cryogenic attenuation has previously been carefully determined to $\Lambda_{\mathrm{c}} = (9.7 \pm 0.7)\,\mathrm{dB}$ in Ref. S1. The microwave output of the sample is connected via three circulators (two at the millikelvin stage and one at the 0.7 K stage) to a cryogenic low-noise amplifier (LNF-LNR4_8) from Low Noise Factory. The circulators shield the nano-electromechanical system from thermal microwave photons originating from the amplifier and the higher lying temperature stages.

To excite a mechanical displacement of the nanostrings, we mount a piezo actuator on the outside of the sample box. This allows for a relatively fast determination of the eigenfrequencies of the mechanical modes, and for the investigation of modes, which are only weakly coupled to the light field.

To tune the resonance frequency of the microwave resonator, we mount a superconducting coil on the top-lid of the sample box. This coil creates a magnetic field oriented roughly perpendicular to the sample surface and allows hereby to tune the inductance of the SQUID. We calibrate the coil using the SQUID's flux periodicity. We find a periodicity of $I_\Phi = 1.17\,\mathrm{mA}$ by using the flux quantum $\Phi_0 = 2.07 \times 10^{-15}\,\mathrm{Tm}^2$. Given the SQUID's dimension with a loop area of $A_{\mathrm{loop}} = 44.6\,\mathrm{\mu m}^2$, we find a current-field relation of $B_{\mathrm{ext}} = (39.8 \pm 0.2)\,\mathrm{mT/A} \cdot I_{\mathrm{coil}}$.

In Fig. S1**b**, we present the room temperature detection setup employed for the thermal noise measurements as well as for the characterization of the frequency tunable microwave resonator. The setup consists of a microwave source, which provides the microwave tone for driving the electromechanical Raman type process, i.e. the scattering of photons to the Stokes and anti-Stokes field. Those are later measured using a spectrum analyser, after down-conversion of the microwave signal with an IQ mixer. For the down-conversion process, we use a local oscillator (LO) with the same frequency as for the incident microwave tone ($\omega_{\mathrm{p}} = \omega_{\mathrm{LO}}$) and add the resulting I and Q quadrature with a $90^\circ$ combiner. This technique removes the necessity to control the phase difference between the microwave source, used as LO, and the probe tone connected to the "signal in" line. In addition, we use a vector network analyser to measure the complex transmission of the microwave resonator prior to every experiment. We then determine the resonance frequency of the microwave resonator and configure the frequency of the microwave source $\omega_{\mathrm{p}}$ accordingly to the desired detuning $\Delta$.

For the experiments investigating the microwave transmission under strong mechanical excitation of the nanostring oscillator, we employ the room-temperature microwave setup sketched in Fig. S1**c**. For this experiment, we connect the microwave source directly to the piezo actuator to drive a mechanical motion of the nanostring ($\omega_{\mathrm{p}} \approx \Omega_{\mathrm{m}}$). We subsequently measure the modified microwave transmission using the vector network analyser.

The sample and the sample box, including the superconducting coil, are mounted in a bulk aluminium capsule. At the temperatures of the experiments, the aluminium capsule is in the superconducting state and acts as a magnetic shield, screening the device against magnetic field noise. The device temperature is measured using a resistive thermometer. In particular, we use a calibrated ruthenium-oxide resistor mounted on the outside of the sample enclosure.

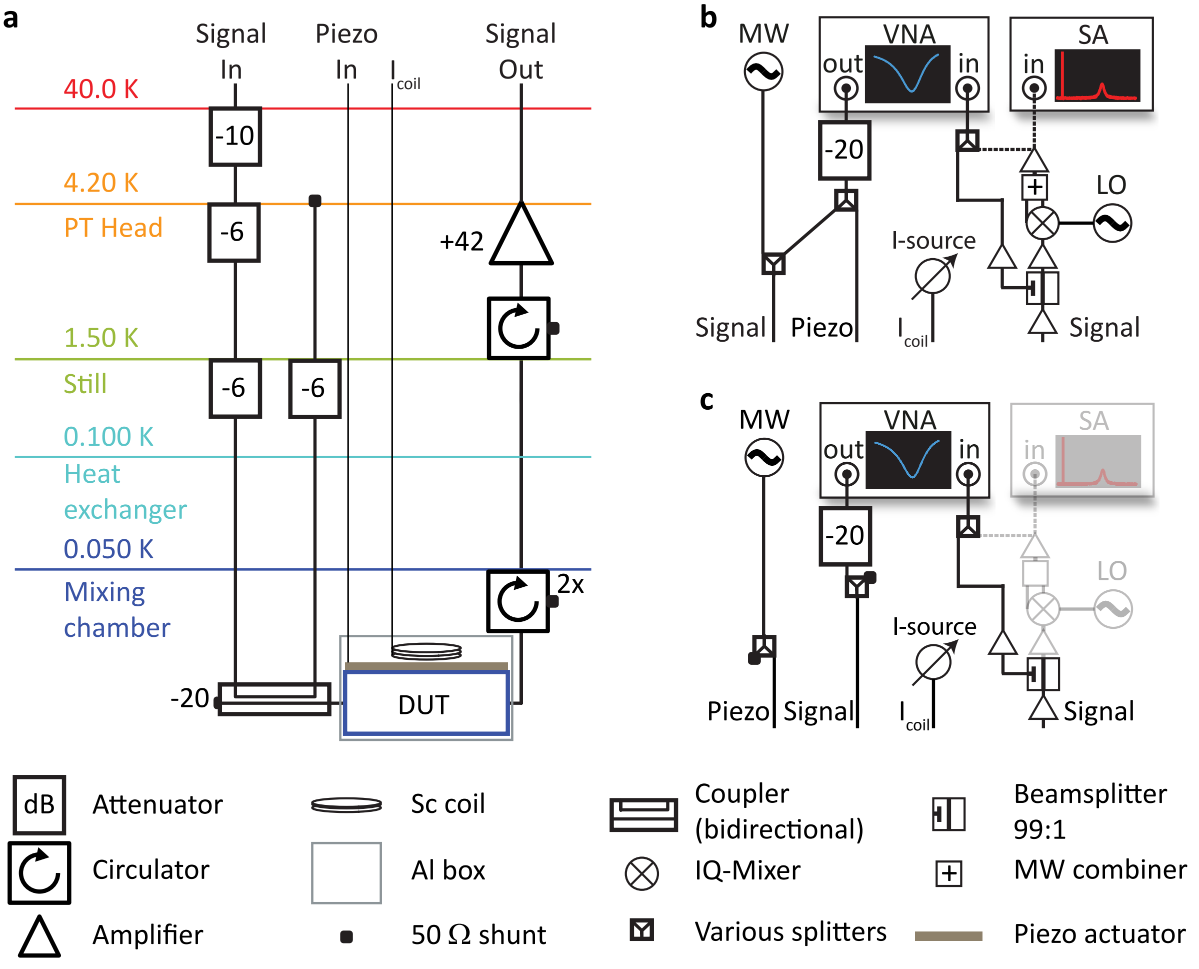


FIG. S1. **Microwave detection setup.** Panel **a** shows the cryogenic part of the microwave setup realising a microwave transmission experiment. The signal input line is equipped with various attenuators to prevent that thermal microwave noise photons from room temperature populate the microwave resonator. The output of the sample box, containing the electromechanic device, is connected to a low noise amplifier via three circulators. In addition, a piezo actuator is mounted on the outside of the sample box to provide a mechanical force for the excitation of the string. A superconducting coil creates the magnetic flux to tune the inductance of the SQUID and hereby the microwave resonance frequency. Panel **b** displays the room temperature microwave setup employed for all experiments besides the experiments presented in Fig. 5 in the main text. The setup for this experiment is separately shown in panel **c**. Further details are provided in the text.

The microwave transmission $|S_{21}|^2$ in Fig. 2**a** in the main text is derived from a combination of directly measured scattering parameters $S_{21}^{\mathrm{meas}}$ with a reference scattering parameter $S_{21}^{\mathrm{mw}}$ for which the tunable resonator is shifted outside the measured frequency range. The displayed absolute transmission is derived as

$$|S_{21}|^2 = \left| \frac{S_{21}^{\mathrm{meas}}}{S_{21}^{\mathrm{mw}}} \right|^2 . \tag{S1}$$

## II. SQUID SHUNTED FREQUENCY TUNABLE MICROWAVE RESONATOR

In this section, we discuss the frequency tuning of the microwave resonator when: (i) a static magnetic flux is applied to the SQUID and (ii), a microwave drive is applied to the microwave resonator (i.e. microwave power induced frequency tuning).

## A. Static magnetic flux induced tuning of the microwave resonance frequency

### 1. The model

The nano-electromechanical hybrid device presented in Fig. 1 in the main text consists of a CPW resonator which is shunted to ground by a dc-SQUID. The CPW part of the microwave resonator can be described in the form of a distributed element coplanar waveguide resonator with a specific inductance and capacitance per unit length of[S2]

$$L_{\mathrm{l}} = \frac{\mu_0}{4}\frac{K(k_0')}{K(k_0)} \text{ and} \tag{S2}$$

$$C_{\mathrm{l}} = 4\epsilon_0\epsilon_{\mathrm{eff}}\frac{K(k_0)}{K(k_0')}. \tag{S3}$$

Here, $K$ is the complete elliptic integral of first kind. The parameters $k_0 = w_{\mathrm{c}}/(w_{\mathrm{c}} + 2s_{\mathrm{c}})$ and $k_0' = \sqrt{1-k_0^2}$ relate to the geometry of the CPW, i.e. the width of the center conductor $w_{\mathrm{c}} = 10\,\mu\mathrm{m}$ and the gap between it and the ground plane $s_{\mathrm{c}} = 8\,\mu\mathrm{m}$. The effective dielectric constant $\epsilon_{\mathrm{eff}}$ in our circuit is 6.45. Hereby, we obtain a line impedance $Z = \sqrt{L_{\mathrm{l}}/C_{\mathrm{l}}} = 56\,\Omega$, with $L_{\mathrm{l}} = 4.80\times10^{-7}\,\mathrm{H/m}$ and $C_{\mathrm{l}} = 1.49\times10^{-10}\,\mathrm{F/m}$. The physical CPW length of $l_{\mathrm{c}} = 2.930\,\mathrm{mm}$ corresponds to a bare microwave resonance frequency of $\omega_0/2\pi = c/(\sqrt{\epsilon_{\mathrm{eff}}}4l_{\mathrm{c}}) = 9.85\,\mathrm{GHz}$. Alternatively, the CPW resonator can also be modeled as an effective LC-circuit [S2] with an capacitance $C_{\mathrm{c}} = C_{\mathrm{l}}l_{\mathrm{c}}/2 = 224\,\mathrm{fF}$ and an inductance $L_{\mathrm{c}} = 8L_{\mathrm{l}}l_{\mathrm{c}}/\pi^2 = 1.17\,\mathrm{nH}$, corresponding to a resonance frequency $\omega_0 = 1/\sqrt{L_{\mathrm{c}}C_{\mathrm{c}}}$ [S3]. The coupling capacitance is estimated to be on the order of 2 fF and therefore, we neglect the impact of the coupling capacitance on the microwave resonance frequency in the following discussion.

The integration of a dc-SQUID in a microwave resonator at a suitable location, such as in our experiment, allows to modify the total inductance of the microwave circuit and hereby enables the tuning of its resonance frequency $\omega_{\mathrm{c}}$. For the particular case of the integration of a dc-SQUID in a distributed CPW resonator, we follow Refs. [S4–S6], where the resonance frequency is given by

$$\frac{\pi\omega_{\mathrm{c}}}{2\omega_0}\tan\left(\frac{\pi\omega_{\mathrm{c}}}{2\omega_0}\right) = \frac{2\pi^2}{\Phi_0^2}L_{\mathrm{c}}E_{\mathrm{s}}(\Phi_{\mathrm{ext}}). \tag{S4}$$

Here, we have introduced the inductive energy of the dc-SQUID as [S6]

$$E_{\mathrm{s}}(\Phi_{\mathrm{ext}}) = \frac{\Phi_0^2}{(2\pi)^2}\frac{1}{L_{\mathrm{J}}(\Phi_{\mathrm{ext}}) + L_{\mathrm{loop}}/4}. \tag{S5}$$

The latter consists of contributions from both Josephson junctions (in total $L_{\mathrm{J}}$) and the geometric loop inductance $L_{\mathrm{loop}}$. For details on the determination of the individual SQUID inductances, we refer to Ref. [S7]. The Josephson inductance of the SQUID is related to the critical current $I_{\mathrm{c}}$ via

$$L_{\mathrm{J}}(\Phi_{\mathrm{ext}}) = \frac{\Phi_0}{4\pi I_{\mathrm{c}}\left|\cos(\pi\Phi_{\mathrm{ext}}/\Phi_0)\right|}. \tag{S6}$$

To explicitly determine the resonator frequency tuning, we expand the left hand side of Eq. (S4) around $\pi/2$ corresponding to $\omega_{\mathrm{c}}/\omega_0 \simeq 1$ around the sweet spot[S8] ($\Phi_{\mathrm{ext}}/\Phi_0 \approx n \in \mathbb{Z}$),

$$\frac{\pi\omega_{\mathrm{c}}}{2\omega_0}\tan\left(\frac{\pi\omega_{\mathrm{c}}}{2\omega_0}\right) = -\frac{1}{\omega_{\mathrm{c}}/\omega_0 - 1} - 1 + \mathcal{O}(\frac{\omega_{\mathrm{c}}}{\omega_0} - 1). \tag{S7}$$

Combining (S7) with (S4) yields the resonance frequency of the microwave resonator as a function of the applied external magnetic flux [S6]

$$\omega_{\mathrm{c}}(\Phi_{\mathrm{ext}}) = \omega_0\left(1 + \frac{L_{\mathrm{J}}(\Phi_{\mathrm{ext}}) + L_{\mathrm{loop}}/4}{L_{\mathrm{c}}}\right)^{-1}. \tag{S8}$$

Note that (S8) assumes $\omega_{\mathrm{c}}/\omega_0 \simeq 1$ that the externally applied flux $\Phi_{\mathrm{ext}}$ is close to the resonator's sweet spot.

The loop inductance of the SQUID consists of geometric and kinetic contributions $L_{\mathrm{loop}} = L_{\mathrm{geo}} + L_{\mathrm{kin}}$. The geometric inductance can be deduced from the SQUID design. For the geometry of our SQUID, we find $L_{\mathrm{geo}} = 19\,\mathrm{pH}$ (Tab. S1 in combination with Ref. [S9]). The kinetic induction of the SQUID originates mainly from the thin and long sections forming the nanostrings. This inductance scales with $l/S$, where S is the string‘s cross section,

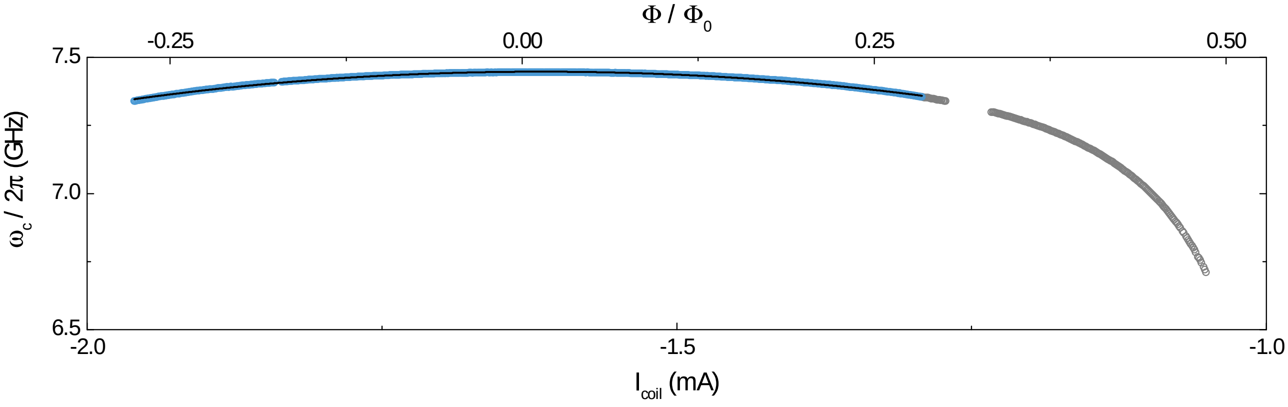


FIG. S2. **Frequency tuning of the microwave resonator by a static magnetic field.** The grey and blue circles show the resonance frequency of the microwave resonator determined from Fig. 2 in the main text as a function of the coil current for a temperature of 85 mK. In addition, the top-axis shows the corresponding effective flux threading the dc-SQUID loop after subtracting a constant flux offset. We find a tuning of the resonance frequency to lower values for flux values deviating from zero, which is expected due to the increase in the inductance of the microwave circuit. For a quantitative analysis of the critical current $I_c$, we fit the data to Eq. (S8) in the frequency range indicated by the blue circles. For more details, we refer to the text.

and pre-characterizations show a prefactor of $4.5 \times 10^{-8}$ pHm for our material system [S10]. Therefore, $L_{\text{kin}} = 4.5 \times 10^{-8}\,\text{pHm} \times l/S = 41\,\text{pH}$. Consequently, the complete loop inductance is $L_{\text{loop}} = 60\,\text{pH}$, which is dominated by the kinetic inductance stemming from the string geometry.

As $L_{\text{loop}}$ and $L_{\text{c}}$ are known, we can use Eq. (S8) to determine the critical current $I_{\text{c}}$ of a single Josephson junction from the experimental data shown in Fig. S2.

We like to note that the microwave circuit could also be modeled as an effective lumped element circuit. However, the accurate description in the form of a distributed element system takes the correct boundary conditions of the electromagnetic field inside the resonator, in particular at the location of the SQUID, into account. In addition, Bourassa et al. [S11] showed that this approach allows to model any strength of the nonlinearity including e.q. the ones present in a transmon qubit.

### *2. Tuning of the resonance frequency using a static magnetic flux bias*

As presented in Figure 2 of the main text, we can tune the resonance frequency of the microwave resonator by applying a static magnetic field, resulting in a static flux bias of the dc-SQUID. For a more quantitative analysis of the data, we extract the resonance frequency by searching for the minimum of the microwave transmission for each magnetic field or coil current. Figure S2 shows the resulting resonance frequency as a function of the coil current in grey and blue circles. We discard the data around a resonance frequency of 7.3 GHz, as here the resonator couples to a parasitic mode.

The data shown in Fig. S2 as well as in Fig. 2 of the main text allows to calibrate the superconducting coil used for the static flux bias. Using the parameters of the SQUID listed in Tab. S1, we find a field calibration of 39.8 mT/A. In addition, we can plot the frequency tuning as a function of the bias flux as shown in the top-axis of Fig. S2.

Furthermore, the data in Fig. S2 allows us to quantify the critical current $I_{\text{c}}$ of the Josephson junctions in the SQUID using Eq. (S8). For our analysis, we restrict ourselves to resonance frequencies close to the sweet spot, to be specific the blue coloured circles in Fig. S2, such that the approximation for the derivation of Eq. (S8) is valid. Hereby, we obtain a critical single-junction current of 442 nA, assuming that the Josephson junctions have an identical critical current. Given the design parameters of the Josephson junctions with a junction area of $A_{\text{JJ}} = 240\,\text{nm} \times 500\,\text{nm}$, we find a critical current density of $368\,\text{A/cm}^2$. Using Eq. (S6), we derive $L_{\text{J}} = 0.360\,\text{nH}$, corresponding to a resonance frequency at the sweet spot of $\omega_{\text{c}}(\Phi_{\text{ext}} = 0)/2\pi = 7.46\,\text{GHz}$. This is in good agreement with the measured value of 7.445 GHz. The Josephson inductance corresponds to a Josephson energy at the sweet spot of $E_{\text{J}}/h = 2I_{\text{c}}\Phi_0/\hbar = 406\,\text{GHz}$. With these parameters, we determine the screening parameter $\beta_{\text{L}} = 2I_{\text{c}}L_{\text{loop}}/\Phi_0 = 0.013$. Thus, we expect and observe a negligible hysteretic behavior of our resonator when sweeping the external magnetic field bias as $\beta_{\text{L}} \ll 1$.

### B. Microwave power induced shift of the resonance frequency

In addition to the linear response regime, the SQUID in the microwave resonator causes a microwave power-dependent shift in the resonance frequency. This shift originates from the fact that a current flowing across the Josephson junction can be associated with a modification of the junction's inductance. Thus, the oscillating microwave current will cause a change in the SQUID inductance and hereby a frequency shift.

We can account for this power or current dependent inductance similar to Refs. S12 and S13 by writing the dc-SQUID inductance as

$$L_{\mathrm{S}}(I,\Phi) = L_{\mathrm{J}} + L_2 (I/I_{\mathrm{c}})^2. \tag{S9}$$

Here, we introduce a parabolic correction term $L_2$. Equation (S8) then reads

$$\omega_{\mathrm{c}}(I,\Phi_{\mathrm{ext}}) = \omega_0 \left(1 + \frac{L_{\mathrm{loop}}}{4L_{\mathrm{c}}} + \frac{L_{\mathrm{J}}}{L_{\mathrm{c}}} + \frac{L_2 (I/I_{\mathrm{c}})^2}{L_{\mathrm{c}}}\right)^{-1}. \tag{S10}$$

Defining $\omega_{\mathrm{c}}^0(\Phi_{\mathrm{ext}}) = \omega_{\mathrm{c}}(0,\Phi_{\mathrm{ext}})$ we can rewrite (S10) to identify the nonlinear response terms. Note that $L_2$ as well as $L_{\mathrm{J}}$ are flux dependent and therefore the degree of nonlinearity of the response will depend on the flux bias point.

$$\omega_{\mathrm{c}}(I,\Phi_{\mathrm{ext}}) = \omega_{\mathrm{c}}^0(\Phi_{\mathrm{ext}}) \left[1 + \frac{L_2}{L_{\mathrm{c}} + L_{\mathrm{loop}}/4 + L_{\mathrm{J}}} \left(\frac{I}{I_{\mathrm{c}}}\right)^2\right]^{-1} \tag{S11}$$

To understand the frequency shift in our experiment, we need to take the specific operation conditions into account (cf. also Sec. II C). We apply a fixed-frequency microwave tone $\omega_{\mathrm{p}}$ resonant with the initial resonance frequency $\omega_{\mathrm{c}}(\Phi_{\mathrm{ext}})$ of the microwave circuit. When increasing the power (up to 19 pW), we observe a shift in the resonance frequency of the microwave resonator to lower frequencies. We measure this shift using a much weaker probe tone (of 6.4 aW) in a two-tone microwave transmission experiment. As shown in Fig. S3**b**, we find a shift of the resonator frequency (the blue feature in the transmission data) to lower values. From this data, we determine the resonance frequency and hereby the shift as a function of the applied microwave power at $\omega_{\mathrm{p}}$ (cf. Fig. S3**d**).

To explain the observed down-shift in the resonance frequency in terms of the nonlinearity discussed above, we need to account for the filter function of the microwave resonator itself. As the incident microwave tone at $\omega_{\mathrm{p}}$ populates the microwave resonator with photons, it affects the inductance of the SQUID via the oscillating current $I$ in the junctions of the SQUID. This tunes the resonance frequency according to (S11). To obtain a measure for this current, we determine the intra-resonator photon number via [S14, S15]

$$\bar{n}_{\mathrm{r}} = \frac{P_{\mathrm{mw}}}{\hbar\omega_{\mathrm{p}}} \frac{4\kappa_{\mathrm{ex}}}{4(\omega_{\mathrm{c}} - \omega_{\mathrm{p}})^2 + \kappa^2} \tag{S12}$$

Solving (S11) and (S12) we obtain

$$\omega_{\mathrm{c}} \approx \omega_{\mathrm{c}}^0 - \left(\frac{L_2}{L_{\mathrm{c}} + L_{\mathrm{J}} + L_{\mathrm{loop}}/4} \frac{c\kappa_{\mathrm{ext}}}{\hbar}\right)^{1/3} P_{\mathrm{mw}}^{1/3} \tag{S13}$$

assuming that the microwave resonator is detuned from its undisturbed frequency by more than one linewidth. Further, $c$ relates the photon number to the current in the SQUID $(I/I_{\mathrm{c}})^2 = c\,\bar{n}_{\mathrm{r}}$.

We find an excellent agreement between the data shown in Fig. S3**d** and the power law predicted by Eq. (S13). In addition, we want to note that the power law describing the shift in the resonance frequency of the microwave resonator is independent of the detailed nature of the flux tunable resonator, i.e. we find the same power law for the case of a frequency tunable lumped element resonator with a dc-SQUID.

### C. Nonlinear flux tuneable microwave resonators

Here, we present the data discussing the nonlinearity of the microwave resonator response, when it is subjected to a microwave tone. We study this nonlinearity using two experimental approaches: (i) we use a single spectroscopy tone (cf. Fig. S3**a**) and (ii) we use a two-tone approach (cf. Fig. S3**b**, **c**).

For the first experimental setting, we perform our experiment by configuring the electromechanical system on working spot K and probe its transmission with a single microwave spectroscopy tone of increasing incident power of

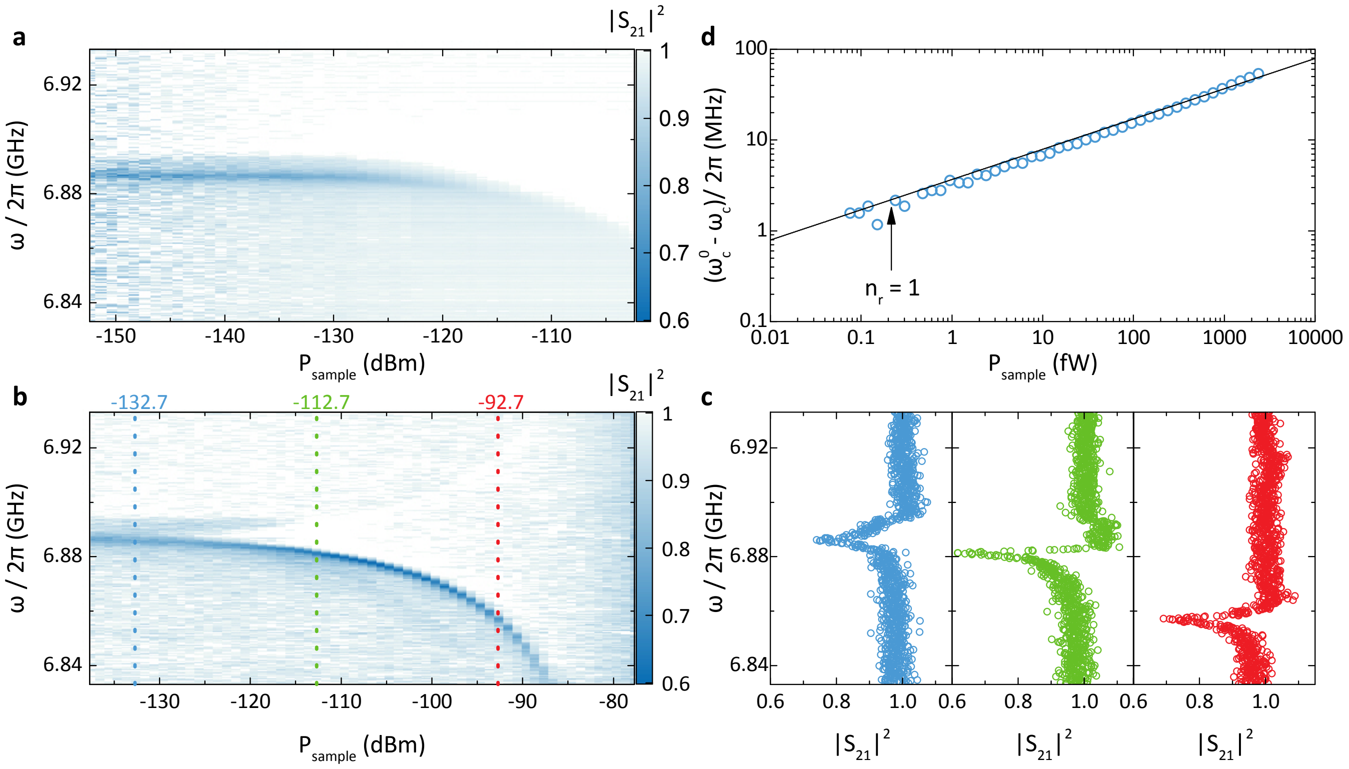


FIG. S3. **Nonlinear response of the microwave resonator under strong microwave drive.** Panel **a** shows the corrected microwave transmission of the electromechanical device, when the system is biased to the working point K and $B_{\mathrm{ext}} = 470\,\mu\mathrm{T}$. The experiment utilises a single spectroscopy tone for each data trace (representing a constant microwave power) from low to high frequencies. For $P_{\mathrm{sample}} > -125\,\mathrm{dBm}$, we find the characteristic nonlinear response of a resonator with a shark-fin line transmission function. This behavior can be modeled with a Duffing-type nonlinearity with a negative prefactor. In addition, we observe a shift of the transmission minimum to lower frequencies. Panel **b** shows a second set of experiments which is closer to the measurement scheme used for the determination of $g_0$. Here, we apply a probe tone of fixed frequency $\omega_{\mathrm{p}}/2\pi = 6.887\,\mathrm{GHz}$ to the device and vary its power $P_{\mathrm{sample}}$. We measure the corrected microwave transmission using a second, weaker spectroscopy tone. The results are shown in panel **b** and **c**, where the latter displays three selected drive tone power values, indicated by their corresponding powers in panel **b**. We find a shift in the transmission signature of the resonator to lower values for increasing drive tone powers $P_{\mathrm{sample}}$ at $\omega_{\mathrm{p}}$. In addition, we observe a slight increase in the transmission, tuning up in frequency. To quantify the shift of the microwave resonator, we extract its resonance frequency $\omega_{\mathrm{c}}(P_{\mathrm{sample}}, \Phi_{\mathrm{ext}})$ by taking the minimum transmission for each drive power. Panel **d** shows the frequency shift $\delta\omega = \omega_{\mathrm{c}}^0(\Phi_{\mathrm{ext}}) - \omega_{\mathrm{c}}(P_{\mathrm{sample}}, \Phi_{\mathrm{ext}})$ as blue circles. In addition, we plot the power law from Eq. (S13) ($P_{\mathrm{sample}}^{1/3}$-dependence) as black solid line and observe an excellent agreement between the data and the model. We also indicate the power equivalent to an average photon number of one in the microwave resonator with an arrow and deduce a single photon frequency shift of about 2 MHz.

up to about 0.1 pW corresponding to $-100\,\mathrm{dBm}$. The corrected microwave transmission data is shown in Fig. S3**a**. For the correction, we take a complex transmission trace as reference for the same frequency span, when the microwave resonator is detuned in frequency. The corrected transmission is then calculated by complex division of the data trace by the reference trace for each frequency point. For the data presented in Fig. S3**a**, we find a Lorentzian lineshape with a minimum at a constant frequency for low drive powers of up to $-125\,\mathrm{dBm}$. Above this power level, we observe a shark-fin like microwave transmission and a shift of the resonance frequency to lower values. This behavior is prototypical for a nonlinear response of the resonator and can be modeled with a Duffing-type negative nonlinearity.[S4]

For the determination of $g_0$, the second experimental approach is of more relevance, as this approach corresponds to the experimental setting used for the microwave excitation of the electromechanical system. Here, we apply a microwave tone with constant frequency $\omega_{\mathrm{p}}$ and vary its intensity. We use an additional, second spectroscopy tone of significantly lower intensity of 19 aW to probe the transmission function of the microwave resonator. The data of this experiment is depicted in Fig. S3**b** for $\omega_{\mathrm{p}}/2\pi = 6.887\,\mathrm{GHz}$. As discussed above, the main feature of the data is a tuning of the resonance frequency of the resonator to lower frequencies. This behavior is analysed in more detail in panel **d** where we quantitatively compare the shift in the resonance frequency $\delta\omega$ with the power law of Eq. (S13)

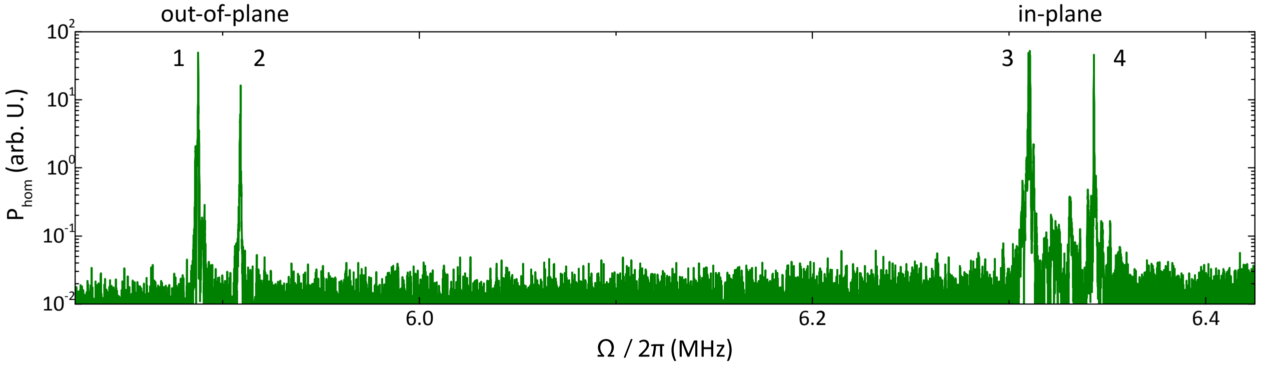


FIG. S4. **Resonance response of the driven mechanical strings.** The overview spectra of the two nanomechanical strings is shown. We find two pairs of modes for the two nanostrings that we assign to the in- and out-of-plane modes. From the string's cross section, the in-plane modes are expected to appear at higher frequencies than the out-of-plane modes. Further experiments confirmed this expectation, as discussed in the main text. Besides this plot, all experiments within this work are performed on mode 4.

and find a frequency shift of $(367 \pm 4)\,\mathrm{GHzW}^{-1/3}$. As stated above, we find an excellent agreement between the data and the model. However, we do not quantitatively relate the observed prefactor to the parameters $L_\mathrm{J}$ and $L_2$ as the proportionality constant $c$ relating the intra-resonator current to the incident microwave power is unknown. This data set also allows to quantify the single photon frequency shift. The probe tone microwave power $P_\mathrm{sample} = 0.2\,\mathrm{fW}$ corresponds to an average photon number of $\bar{n}_\mathrm{r} \approx 1$ taking the resonator filter function into account. This power level is indicated by the black arrow in Fig. S3**d**. Here, we deduce a single photon frequency shift of 2.2 MHz.

In addition to the shift in the resonance frequency, we observe an increase in the transmission tuning to higher frequencies in Fig. S3**b**. We attribute this to the interference of the two microwave tones. Similar features have been reported in strongly driven systems.[S16] In panel **c** we show the corresponding transmission close to the microwave resonator's eigenfrequency for selected incident drive powers ($-132.7\,\mathrm{dBm}$, $-112.7\,\mathrm{dBm}$, and $-92.7\,\mathrm{dBm}$). In addition to the frequency tuning, here we observe that the depth of the absorption in resonance changes slightly. We attribute this to the change in the total inductance of the microwave resonator which in turn affects the coupling $\eta$. In particular, the impedance of the microwave resonator is affected by the change in the inductance, resulting in a change in the matching conditions.

## III. MECHANICAL MODES OF THE SUSPENDED SQUID

For the suspension of the nanostring oscillators, we perform a reactive ion etching step on the entire chip. Therefore, both SQUID arms are freely suspended as shown in Fig. 1 in the main text. In this respect, we expect the excitation of multiple mechanical resonances and modes with different symmetry.

For the experimental investigation of the mechanical modes, we configure the microwave resonator at working point K and an external field bias of $B_\mathrm{ext} = -462\,\mu\mathrm{T}$. The temperature is 111 mK. We use the setup depicted in Fig. S1**a**, and **b**, where we probe the mechanical response via the microwave resonator ($\omega_\mathrm{p} = \omega_\mathrm{c}$) while driving the piezo actuator actively at the frequency $\Omega$ using the network analyser. This measurement concept has the benefit, that it enables a fast detection of all mechanical modes, even if the modes are only weakly coupled to the microwave resonator. [S17] However, we would like to note, that due to the relatively large detection bandwidth of 20 Hz chosen for this experiment, the amplitude $P_\mathrm{hom}$ does not represent a good measure for the coupling strength. Figure S4 displays the mechanical response as function of the mechanical excitation frequency $\Omega$. We detect four dominant peaks in the spectrum at

$$\begin{aligned}\Omega_{\mathrm{m},1}/2\pi &= 5.887\,58\,\mathrm{MHz},\\ \Omega_{\mathrm{m},2}/2\pi &= 5.909\,24\,\mathrm{MHz},\\ \Omega_{\mathrm{m},3}/2\pi &= 6.310\,28\,\mathrm{MHz},\ \text{and}\\ \Omega_{\mathrm{m},4}/2\pi &= 6.343\,16\,\mathrm{MHz}.\end{aligned}$$

Regarding the assignment of the modes to specific geometric excitations, we can differentiate two scenarios: (i) The nanostrings do not couple and the mode frequencies differ by more than their linewidth, because of the length

variation between the strings and their approximately rectangular cross-section. (ii) The second case is a coupled-string scenario similar to reports in Ref. [S18–S21], where the mechanical modes of the strings hybridise as they are sharing at least one clamping point.

We start the discussion with scenario (i). Here, in the uncoupled case, the resonance frequency of the fundamental mode of a tensile-stressed string is given by [S22–S24]

$$\Omega_{\mathrm{m}} = \frac{\pi^2}{l^2}\sqrt{\frac{E_{\mathrm{Y}} I_{\mathrm{m}}}{\rho S}}\sqrt{1+\frac{\sigma S l^2}{E_{\mathrm{Y}} I_{\mathrm{m}} \pi^2}} \approx \frac{\pi}{l}\sqrt{\frac{\sigma}{\rho}}, \tag{S14}$$

where the approximation assumes highly tensile stressed strings

$$\frac{E_{\mathrm{Y}} I_{\mathrm{m}} \pi^2}{S l^2} \ll \sigma. \tag{S15}$$

Here, $l$ and $S$ are the length and the cross-sectional area of the mechanical string resonator, $\rho$ is the density of the material, $\sigma$ is the tensile stress of the string provided by the clamping, $E_{\mathrm{Y}}$ is the Young's modulus of the material, and $I_{\mathrm{m}}$ is the moment of inertia, which depends on the geometry of the string. For the in-plane and out-of-plane motion, the moments of inertia differ due to the approximately rectangular shape of the string's cross-section. In particular, the moment of intertia is $I_{\mathrm{m}}^{\mathrm{ip}} = w^3 t/12$ for the in-plane and $I_{\mathrm{m}}^{\mathrm{oop}} = w t^3/12$ for the out-of-plane mode. Therefore, the in-plane mode should have a higher resonance frequency compared to the out-of-plane mode. Indeed, the mode investigated in the main text (mode 4) has the highest resonance frequency, suggesting that it corresponds to an in-plane displacement. Moreover, additional measurements indicate that mode 3 and mode 4 have a higher electromechanical coupling rate than mode 1 and 2 suggesting that mode 3 and 4 are the modes with a larger in-plane displacement. We therefore relate later to mode 1 and 2 as the out-of-plane modes and mode 3 and 4 as the in-plane modes.

Next, we turn to a quantitative analysis of the mechanical parameters. For the determination of the pre-stress we use the approximated form of Eq. (S14). Using the design parameter $l = 20\,\mu\mathrm{m}$ and the resonance frequency $\Omega_{\mathrm{m},4}$ of mode 4, we obtain $\sigma = 174\,\mathrm{MPa}$. This also corroborates, that the mechanical resonator can be reasonably approximated as high-tensile stressed string as $E_{\mathrm{Y}} I_{\mathrm{m}} \pi^2/(S l^2) = 5.8\,\mathrm{MPa} \ll \sigma$. Here, we use a Young's modulus of 70 GPa for aluminium[S25]. Given the estimate for $\sigma$, we can use the information about the various mechanical resonance frequencies of the modes to estimate the length difference between the two strings. E.g. assuming that $\Omega_{\mathrm{m},3}$ represents the in-plane mode of the second string, we find a length difference of 100 nm between the strings. Given the huge aspect ratio of the structure, a length difference of 100 nm is certainly within the limits of the electron beam lithography tool used to define structures.

Furthermore, we can employ the exact form of Eq. (S14) for a coarse estimate of the frequency difference between the in- and out-of-plane modes, where we note that Eq. (S14) uses a hinged boundary condition for connecting the string to the clamps.[S22] Using the parameters summarised in Tab. S1, we find for the in-plane mode 4 a tensile-stress of $\sigma = 168.1\,\mathrm{MPa}$. The corresponding out-of-plane mode of the same string is then expected at $\Omega_{\mathrm{m},2}/2\pi = 6.2702\,\mathrm{MHz}$. Although the shift to lower frequencies predicts the trend correctly, it quantitatively differs significantly from the observed resonance frequencies at $\Omega_{\mathrm{m},1}$ and $\Omega_{\mathrm{m},2}$. We attribute this discrepancy to the incorrect treatment of the boundary conditions at the clamps in Eq. (S14).

Next, we turn to numerical simulations of the mechanics of the structure. Hereby, we assess whether the two strings are mechanically coupled via their shared support. In detail, we use the finite element suite COMSOL© for simulating the mechanical aspects of the SQUID. We model the geometry of the SQUID from the design and estimate the 'overhang' of the aluminium layer from Fig. 1**c** (cf. main text). We further define a tensile stress along the x-axis (cf. Fig. S5) of 170 MPa in the aluminium layer. The bottom surface of the silicon support structure is considered a fixed boundary. Under these conditions, we find for the two lowest resonance frequencies 6.7799 MHz and 6.7817 MHz for the out-of-plane modes as well as 7.3504 MHz and 7.3525 MHz for the in-plane modes. The difference of the out-of-plane (in-plane) resonance frequencies is attributed to the slightly different geometry of the clamps, as we set the length of the strings identical in this simulation. This is a good indication, that minimal asymmetries in the support structure detune the resonance frequencies of the mechanical modes sufficiently to prevent a coupling. The frequency difference between the in-plane and out-of-plane modes is more significant compared to the analytic results presented above. Here, we find in the finite element simulations, that the in-plane modes are situated at considerably higher frequencies. This result is naturally understood as the finite element simulation also accounts the bending of the structure present at the clamps, where an out-of-plane motion is less rigidly constrained compared to the in-plane motion. Quantitatively, we observe a frequency difference in the experimental data of 420 kHz which is in good agreement with the finite element modeling predicting a difference of 570 kHz. We attribute the remaining discrepancy to the details in the exact geometry of the clamp and its 'overhang'.

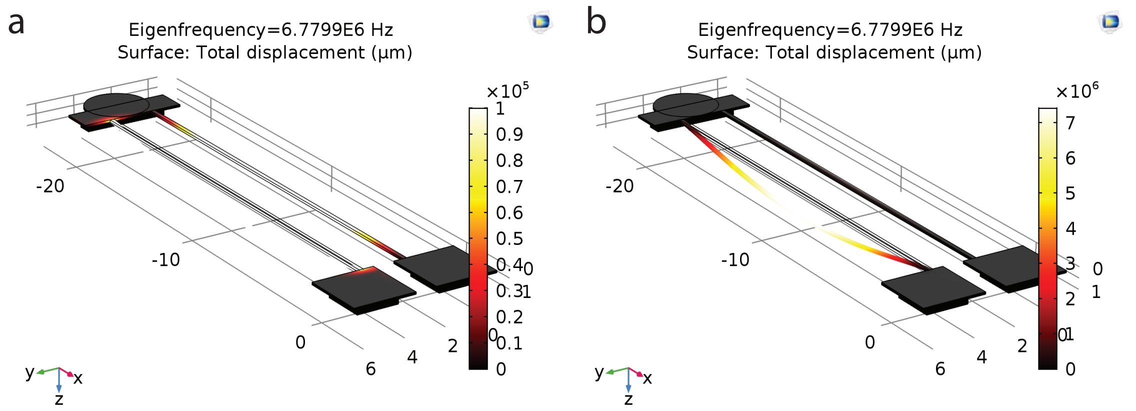


FIG. S5. **Modeled resonance frequency of the nanostrings using COMSOL©.** The panels show the eigenmode with a resonance frequency of 6.78 MHz. Panel **a** shows the simulated displacement amplitude of the suspended structure in arbitrary units. In addition, panel **b** shows the same data, where we changed the scale to focus on the displacement distribution in the clamp. We find that the clamps do not visibly contribute to a mode overlap, suggesting only a minimal coupling.

In summary, the analytical estimate as well as the COMSOL© finite element simulations suggest that our sample can be understood in terms of two uncoupled (or at least weakly coupled) strings. This is in agreement with reports in Refs. [S18–S21] where the authors optimized, and miniaturised the shared clamp in order to achieve the strong coupling regime.

## IV. MEASUREMENT OF THE ELECTROMECHANICAL COUPLING CONSTANT

For the determination of the electromechanical coupling constant, we use a scheme modified from the calibration tone technique discussed by Gorodetsky et al. in Ref. S26. In particular, we use the microwave detection scheme shown in Fig. S1**b**, where we frequency modulate the microwave source to generate the calibration tone. We down-convert the signal coming from the dilution fridge with an unmodulated local oscillator and perform a spectrum analysis of the down-converted signal. This results in the spectra shown in Fig. S6**b**. For a quantitative analysis of this data, we need to obtain information about the transfer functions involved as well (cf. Fig. S6**a**).

The mechanical displacement power spectral density in thermal equilibrium is given by (cf. e.g. Eq. (7) in Ref. S26 or Ref. S14)

$$S_{\mathrm{xx}}^{\mathrm{th}}(\Omega) = \frac{1}{m_{\mathrm{eff}}} \frac{2\Gamma_{\mathrm{m}} k_{\mathrm{B}} T}{(\Omega^2 - \Omega_{\mathrm{m}}^2)^2 + \Gamma_{\mathrm{m}}^2 \Omega^2}. \tag{S16}$$

In nano-electromechanics, the thermal motion of the mechanical element is converted into a frequency shift of the microwave resonator. Hence,

$$S_{\omega\omega} = G^2 S_{\mathrm{xx}} \tag{S17}$$

where $G = g_0/x_{\mathrm{zpm}}$. Therefore, the frequency fluctuations of the microwave resonator can be associated with the number of phonons populating the mechanical element (cf. e.g. Eq. (9) in Ref. S26)

$$\langle \delta\omega^2 \rangle = \int_{-\infty}^{\infty} S_{\omega\omega}(\Omega) \frac{d\Omega}{2\pi} = S_{\omega\omega}(\Omega_{\mathrm{m}}) \frac{\Gamma_{\mathrm{m}}}{2} = 2\bar{n}_{\mathrm{m}} g_0^2. \tag{S18}$$

The next step is to relate the physical observable of the microwave resonator's resonance frequency fluctuations $S_{\omega\omega}(\Omega)$ or phase fluctuations $S_{\Psi\Psi}(\Omega)$ to the measured observable $S_{\mathrm{UU},\Psi}(\Omega_{\mathrm{m}})$ by introducing the transfer function $K_\Psi$ [S27]

$$S_{\mathrm{UU},\Psi}(\Omega) = K_\Psi(\Omega) S_{\Psi\Psi}(\Omega) = \frac{K_\Psi(\Omega)}{\Omega^2} S_{\omega\omega}(\Omega)\,. \tag{S19}$$

In additon, and we formaly distinguish between these transfer functions, the phase calibration tone is converted into a measured signal via

$$S_{\mathrm{UU},\Phi}(\Omega) = K_\Phi(\Omega) S_{\Phi\Phi}(\Omega) \tag{S20}$$

with the transfer function $K_\Phi$. Gorodetsky shows in Ref. S26, that $K_\Phi = K_\Psi$ for the specific cases of a power detection and for the case of optical homodyning. In addition, the measurement apparatus itself has to be taken into consideration. The spectrum analysers used for the detection of the signals perform a discrete Fourier transform of time domain data. The data can be seen as being convoluted with a filter function, which eventually takes the finite bandwidth of the spectrum analyser into account. According to Gorodetsky et al. S26

$$S_{\mathrm{UU}}(\Omega) = 2 \cdot F(\Omega) \star \left( K_\Psi(\Omega) S_{\Psi\Psi}(\Omega) + K_\Phi(\Omega) S_{\Phi\Phi}(\Omega) \right), \tag{S21}$$

where $F(\Omega)$ is the above mentioned filter function with the property

$$F(0) \cdot \mathrm{ENBW} = \int_{-\infty}^{\infty} F(\Omega) \frac{d\Omega}{2\pi} = 1. \tag{S22}$$

The calibration tone detected with the spectrum analyser at the frequency $\Omega_{\mathrm{mod}}$ is[S26]

$$S_{\mathrm{UU},\Phi}(\pm\Omega_{\mathrm{mod}}) \approx \frac{\phi_0^2}{2} \frac{K_\Phi(\Omega_{\mathrm{mod}})}{\mathrm{ENBW}}. \tag{S23}$$

Here we use the phase modulation depth $\phi_0 = \Omega_{\mathrm{dev}}/\Omega_{\mathrm{mod}}$, the modulation frequency $\Omega_{\mathrm{mod}}$, and the measurement bandwidth of the spectrum analyser ENBW in units of Hz. At the mechanical frequency, we expect

$$S_{\mathrm{UU},\Psi}(\Omega_{\mathrm{m}}) = 2K_\Psi(\Omega_{\mathrm{m}}) S_{\Psi\Psi}(\Omega_{\mathrm{m}}) = 2\frac{K_\Psi(\Omega_{\mathrm{m}})}{\Omega^2} S_{\omega\omega}(\Omega_{\mathrm{m}}) = 2\frac{K_\Psi(\Omega_{\mathrm{m}})}{\Omega^2} g_0^2 \frac{4}{\Gamma_{\mathrm{m}}} n_{\mathrm{m}}. \tag{S24}$$

Here, $\Gamma_{\mathrm{m}}$ is the linewidth of the mechanical system and $n_{\mathrm{m}}$ the average phonon number. Thus, we can determine the electromechanical coupling strength by

$$g_0^2 = \frac{\Omega_{\mathrm{m}}^2 \Gamma_{\mathrm{m}}/4}{n_{\mathrm{m}} K_\Psi(\Omega_{\mathrm{m}})} S_{\mathrm{UU},\Psi}(\Omega_{\mathrm{m}}). \tag{S25}$$

Note that this requires knowledge about the transfer function $K_\Psi(\Omega_{\mathrm{m}})$. Gorodetsky et al. S26 showed that for the case of optical power detection and optical homodyning $K_\Psi = K_\Phi$ and determine $g_0$ independently of the transfer functions. We generalize the discussion by introducing the function $\mathcal{Y}$ via

$$K_\Psi = \mathcal{Y} K_\Phi. \tag{S26}$$

Then Eq. (S25) can be expressed in the form

$$g_0^2 = \frac{\phi_0^2 \Omega_{\mathrm{m}}^2 \Gamma_{\mathrm{m}}/4}{n_{\mathrm{m}} \mathcal{Y}\, 4\, \mathrm{ENBW} S_{\mathrm{UU}}(\Omega_{\mathrm{mod}})} S_{\mathrm{UU}}(\Omega_{\mathrm{m}}) = \frac{1}{2n_{\mathrm{m}}} \frac{\Omega_{\mathrm{m}}^2 \phi_0^2}{2} \frac{\Gamma_{\mathrm{m}}}{4} \frac{1}{\mathcal{Y}} \frac{1}{\mathrm{ENBW}} \frac{S_{\mathrm{UU}}(\Omega_{\mathrm{m}})}{S_{\mathrm{UU}}(\Omega_{\mathrm{mod}})}. \tag{S27}$$

Here, we assume $\Omega_{\mathrm{m}} \approx \Omega_{\mathrm{mod}}$, but not $\Omega_{\mathrm{m}} = \Omega_{\mathrm{mod}}$ to prevent an overlap of the two signals. Moreover, $\mathcal{Y}$ needs to be sufficiently constant in the frequency range between $\Omega_{\mathrm{m}}$ and $\Omega_{\mathrm{mod}}$, which is typically satisfied as the frequency difference is mostly small.

### A. Determination of the resonator transfer functions

Next, we need to compute the transfer functions for our microwave down-conversion and detection scheme. For this, we refer to an input-output formalism. The output signal $s_{\mathrm{out}}$ of a cavity or microwave resonator, that is coupled to a transmission line, is described equivalently for both the optical and microwave domain. According to Ref. S26, the intra-resonator field $a_x$ of an electromechanical system, where the mechanical element oscillates with $x(t) = x_0 \cos(\Omega_{\mathrm{m}} t)$, becomes phase modulated with $\psi_0 = x_0 G/\Omega_{\mathrm{m}}$. In detail, the intra-resonator field reads

$$a_x = s_{\mathrm{in}} \sqrt{\eta_{\mathrm{c}} \kappa} \mathcal{L}(0) \left( 1 - \frac{i\psi_0 \Omega_{\mathrm{m}}}{2} \mathcal{L}(+\Omega_{\mathrm{m}}) e^{-i\Omega_{\mathrm{m}} t} - \frac{i\psi_0 \Omega_{\mathrm{m}}}{2} \mathcal{L}(-\Omega_{\mathrm{m}}) e^{+i\Omega_{\mathrm{m}} t} \right). \tag{S28}$$

Note that this expression already accounts for the transfer function of the resonator

$$\mathcal{L}(\Omega) = \frac{1}{-i(\Delta+\Omega)+\kappa/2}, \tag{S29}$$

where $\Delta$ is the detuning of the probe tone from the resonance frequency of the resonator, and $\kappa$ denotes the FWHM of the microwave resonator. The output signal including the encoded motion of the mechanical element is then given by

$$s_{x,\mathrm{out}} = s_{\mathrm{in}} - \sqrt{\eta_c\kappa}\; a_x. \tag{S30}$$

Here, $s_{\mathrm{in}}$ is the unmodulated input signal.[S28]
For a phase modulated input tone ($\phi_0\cos(\Omega_{\mathrm{mod}}t)$) the input signal is [S26]

$$s_{\phi,\mathrm{in}} = s_{\mathrm{in}}\left(1 - \frac{i\phi_0}{2}e^{-i\Omega_{\mathrm{mod}}t} - \frac{i\phi_0}{2}e^{+i\Omega_{\mathrm{mod}}t}\right), \tag{S31}$$

where $\Omega_{\mathrm{mod}}$ is the modulation frequency. The intra-resonator field and the output-field for this particular input tone are

$$a_\phi = s_{\mathrm{in}}\sqrt{\eta_c\kappa}\left(\mathcal{L}(0) - \frac{i\phi_0}{2}\mathcal{L}(+\Omega_{\mathrm{mod}})e^{-i\Omega_{\mathrm{mod}}t} - \frac{i\phi_0}{2}\mathcal{L}(-\Omega_{\mathrm{mod}})e^{+i\Omega_{\mathrm{mod}}t}\right), \text{ and} \tag{S32}$$

$$s_{\phi,\mathrm{out}} = s_{\phi,\mathrm{in}} - \sqrt{\eta_c\kappa}\; a_\phi. \tag{S33}$$

The microwave homodyne/heterodyne detection scheme uses a mixing process to transform the signal $s_{x,\mathrm{out}}$ and $s_{\phi,\mathrm{out}}$ to an intermediate frequency in the MHz range. Using the setup discussed in Sec. I, the voltage present at the I and Q output of the mixer is given by

$$U_{(x,\phi)} = A s_{\mathrm{LO}} s_{(x,\phi),\mathrm{out}}, \tag{S34}$$

where we have introduced the local oscillator signal $s_{\mathrm{LO}}$ and an amplitude factor $A$, which summarises all amplification factors as well as conversion efficiencies. For the down-conversion process, we set $\omega_{\mathrm{LO}} = \omega_{\mathrm{p}}$ and restrict the derivation to an ideal mixing process in the sense of Eq. (S34). For the spectral density at the mechanical resonance frequency, we obtain

$$S_{\mathrm{UU},\Psi}(\Omega_{\mathrm{m}}) = (\hbar\omega_{\mathrm{p}})^2 \frac{8\pi A^2\eta^2\kappa^2\psi_0^2\Omega_{\mathrm{m}}^2 s_{\mathrm{in}}^4}{(4\Delta^2+\kappa^2)\,(4(\Delta-\Omega_{\mathrm{m}})^2+\kappa^2)}. \tag{S35}$$

Defining the transfer function in analogy to Ref. S26, we can write

$$\tilde{K}^{\mathrm{x,U}}(\Omega_{\mathrm{m}}) = \frac{S_{\mathrm{UU},\Psi}}{P_{\mathrm{in}}^2 S_{\psi\psi}} \tag{S36}$$

$$= \frac{16\pi^2A^2\eta^2\kappa^2\Omega_{\mathrm{m}}^2}{(4\Delta^2+\kappa^2)\,(4(\Delta-\Omega_{\mathrm{m}})^2+\kappa^2)}. \tag{S37}$$

For the phase modulated calibration tone, we obtain

$$S_{\mathrm{UU},\phi}(\Omega_{\mathrm{mod}}) = (\hbar\omega_0)^2 \frac{\pi A^2\phi_0^2 s_{\mathrm{in}}^4\left(4(\Delta-\Omega_{\mathrm{mod}})^2+(1-2\eta)^2\kappa^2\right)}{2\,(4(\Delta-\Omega_{\mathrm{mod}})^2+\kappa^2)} \tag{S38}$$

and thus

$$\tilde{K}^{\phi,\mathrm{U}}(\Omega_{\mathrm{mod}}) = \frac{S_{\mathrm{UU},\phi}}{P_{\mathrm{in}}^2 S_{\phi\phi}} \tag{S39}$$

$$= \frac{A^2\left(4(\Delta-\Omega_{\mathrm{mod}})^2+(1-2\eta)^2\kappa^2\right)}{4(\Delta-\Omega_{\mathrm{mod}})^2+\kappa^2}. \tag{S40}$$

Therefore, we obtain $\mathcal{Y}$ by using Eq. (S26)

$$\mathcal{Y} = \frac{16\eta^2\kappa^2\Omega_{\mathrm{m}}^2\left(4(\Delta-\Omega_{\mathrm{mod}})^2+\kappa^2\right)}{(4\Delta^2+\kappa^2)\,(4(\Delta-\Omega_{\mathrm{m}})^2+\kappa^2)\,(4(\Delta-\Omega_{\mathrm{mod}})^2+(1-2\eta)^2\kappa^2)} \tag{S41}$$

$$\approx \frac{16\eta^2\kappa^2\Omega_{\mathrm{m}}^2}{(4\Delta^2+\kappa^2)\,(4(\Delta-\Omega_{\mathrm{m}})^2+(1-2\eta)^2\kappa^2)}. \tag{S42}$$

Here, we choose $\Omega_{\mathrm{mod}} \approx \Omega_{\mathrm{m}}$ as in the experiment.

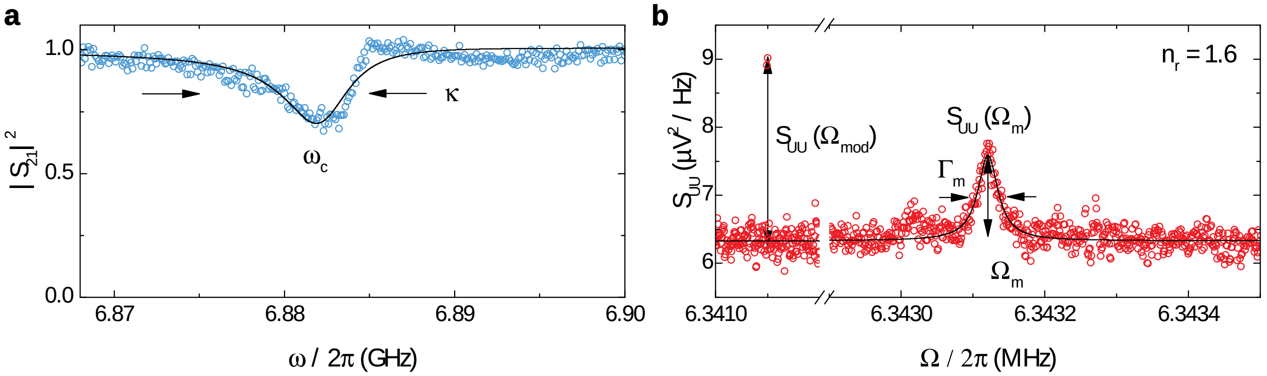


FIG. S6. **Microwave spectroscopy of the thermal mechanical motion.** Panel **a** shows the microwave transmission data using a weak spectroscopy tone, while the microwave probe tone is set to $\omega_\mathrm{p} = \omega_\mathrm{c} + \Omega_\mathrm{m}$ for a temperature $T = 185\,\mathrm{mK}$. This allows to measure the transmission characteristic of the microwave resonator using the same settings as in panel **b**. Panel **b** displays the down-converted scattered microwaves in the vicinity of the mechanical sideband (Stokes field). At $\Omega \approx \Omega_\mathrm{m}$, we find the mechanical signature with a linewidth $\Gamma_\mathrm{m}/2\pi = 34\,\mathrm{Hz}$. Additionally, we use a phase modulation technique resulting in a peak at $\Omega/2\pi = \Omega_\mathrm{mod}/2\pi = 6.3411\,\mathrm{MHz}$ with the amplitude $S_\mathrm{UU}(\Omega_\mathrm{mod})$.

### B. Experimental realization of a $g_0$ measurement.

In this section, we present the quantitative analysis of the microwave resonator and show how the calibration factor $\mathcal{Y}$ is quantitatively determined. We start with the recorded spectra of the microwave resonator and the nanostring oscillator and describe how we extract the parameters relevant for the calibration of $g_0$. We include back-action induced heating effects of the nanostring in the discussion, which we find to be on a negligible level. Repeating the measurements for various temperatures allows us to determine the electromechanical vacuum coupling strength $g_0$.

Figure S6 shows the microwave transmission as well as the noise response attributed to the mechanical motion of the nanostring at flux bias point K and $B_\mathrm{ext} = -470\,\mathrm{\mu T}$. Here, we record the microwave transmission through the device using a weak spectroscopy tone while having a second microwave tone present at $\omega_\mathrm{p} = \omega_\mathrm{c} + \Omega_\mathrm{m}$ with an input power of 5.4 fW. We later use this second tone to scatter microwave photons in the electromechanical sideband using a Raman-type scattering process. By employing the probe tone simultaneously with the spectroscopy tone, we can guarantee that we record the correct microwave transmission function for the analysis presented in Sec. IV A. This is required since the microwave probe tone can affect the characteristics of the microwave resonator as discussed in Sec. II B. The data presented in Fig. S6**a** is corrected by a linear transmission background modeling the microwave transmission of the setup which varies with frequency and temperature and is e.g. caused by cable resonances. We find a characteristic absorption feature at 6.882 GHz. For a quantitative analysis we rely on Eq. (S30). Neglecting, the motion of the string, we can write for the transmission function of the device

$$|S_{21}|^2 = \left|\frac{s_\mathrm{out}}{s_\mathrm{in}}\right|^2 = (\mathrm{o1} - i\,(\mathcal{K}))\,(\mathrm{o1} + i\bar{\mathcal{K}}), \tag{S43}$$

with

$$\mathcal{K} = \mathrm{o2} + \frac{2\eta\kappa}{2\Delta + i\kappa}. \tag{S44}$$

Here, we additionally add a constant complex background accounting for the interference between the on-chip ideal device transmission and undesired port-to-port transmission. In addition, we normalize the complex background by $\mathrm{o2} = \sqrt{1 - \mathrm{o1}^2}$. For the data set in Fig. S6**a**, we determine the following parameters: $\omega_\mathrm{c}/2\pi = 6.882\,\mathrm{GHz}$, $\kappa/2\pi = 4.64\,\mathrm{MHz}$, $\eta = 0.082$, and $\mathrm{o1} = 0.966$, which utilized for the calculation of the black solid line. We speculate that slight deviations between the data and the fit arise from the (complex) background calibration. Given the experimental configuration ($\Delta = +\Omega_\mathrm{m}$), we obtain $\mathcal{Y} = 0.034$ for the data set in Fig. S6**a** using Eq. S42. In our experiments, we also vary the probe-tone power applied at $\omega_\mathrm{p}$ between 2.7 fW and 5.4 fW. In this power regime, the transmission function of the microwave resonator only slightly changes and we can determine an averaged $\mathcal{Y} = 0.031 \pm 0.004$ (cf. also Fig. S8**a**.

The mechanical displacement noise $S_\mathrm{xx}$ manifests itself in the form of a frequency dependent voltage noise at the mechanical frequency $\Omega_\mathrm{m}$ in the down-converted microwave signal. In particular, we detect the voltage fluctuations of

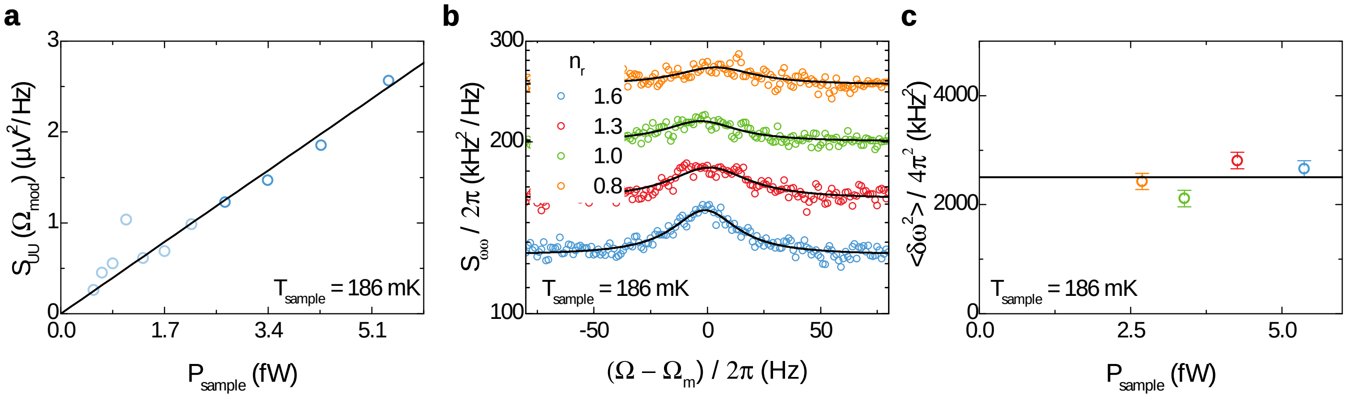


FIG. S7. **Mechanical sideband spectroscopy at $T_{\mathbf{sample}} = 186\,\mathrm{mK}$.** Panel **a** plots the extracted modulation tone peak height $S_{\mathrm{UU}}(\Omega_{\mathrm{mod}})$ (cf. Fig. S6) as a function of the probe tone power showing a linear scaling. The investigated power range from 2.7 fW to 5.4 fW is highlighted, while the power range excluded from the measurement, but confirming the linear behavior, is semi-transparent. In panel **b** we show the frequency spectral density of the microwave resonator caused by the motion of the nanostring. Here, we convert the voltage fluctuations (cf. Fig. S6**b**) to frequency fluctuations using the corresponding calibration tone amplitude $S_{\mathrm{UU}}(\Omega_{\mathrm{mod}})$ and the conversion function $\mathcal{Y}$. For increasing microwave drive amplitudes, the background decreases indicating an imprecision limited detection. The peak area attributed to the mechanical motion ($\langle\delta\omega^2\rangle = S_{\omega\omega}(\Omega_{\mathrm{m}})\Gamma_{\mathrm{m}}/2$) is determined from the data in panel **b** is shown in panel **c** as function of the probe tone power. We find that the integrated frequency fluctuations are probe power independent indicating that the powers used are not significantly affecting the phonon occupation of the mechanical element.

the IQ-Mixer using a spectral analyser with a measurement bandwidth ENBW = 1 Hz. For the generation of the mechanical sidebands at $\omega_{\mathrm{p}} \pm \Omega_{\mathrm{m}}$, we use a probe tone power of 5.4 fW. Figure S6**b** shows the voltage noise spectral power density detected with the spectrum analyser. We find a modulation tone amplitude of $S_{\mathrm{UU}}(\Omega_{\mathrm{mod}}) = 2.56\,\mathrm{\mu V^2/Hz}$ detected at $\Omega = 6.3411\,\mathrm{MHz}$, and a background noise level of $6.34\,\mathrm{\mu V^2/Hz}$. The calibration tone amplitude corresponds to a phase modulation $\phi_0 = 3.94 \cdot 10^{-4}$. For a quantitative analysis of the mechanical displacement spectrum, we fit the data in Fig. S6**b** with Eq. (S16) including an amplitude scaling factor. We find a mechanical displacement noise amplitude of $S_{\mathrm{UU}}(\Omega_{\mathrm{m}}) = 1.26\,\mathrm{\mu V^2/Hz}$, and a mechanical linewidth $\Gamma_{\mathrm{m}}/2\pi = 33.6\,\mathrm{Hz}$. Using these parameters and Eq. (S27), we estimate for the electromechanical coupling strength

$$g_0/2\pi = 1456\,\mathrm{Hz}. \tag{S45}$$

Note, that the latter value assumes that the nanostring is in thermal equilibrium with its environment at $T = 186\,\mathrm{mK}$ corresponding to an average phonon number of $\bar{n}_{\mathrm{m}} = k_{\mathrm{B}}T/\hbar\Omega_{\mathrm{m}} = 612$. However, we perform the experiment with the probe tone set to $\omega_{\mathrm{p}} \approx \omega_{\mathrm{c}} + \Omega_{\mathrm{m}}$, i.e. the blue sideband configuration. Therefore, we need to discuss potential sources of back-action. We experimentally address this point by measuring the mechanical displacement noise as function of the probe-tone power and function of the temperature.

Figure S7**a** shows $S_{\mathrm{UU}}(\Omega_{\mathrm{mod}})$ as function of the probe tone power for $T = 186\,\mathrm{mK}$, where we find the expected linear scaling. Combining this with the knowledge about $\mathcal{Y}$, enables us to convert the spectra recorded in $S_{\mathrm{UU}}$ to $S_{\omega\omega}$ via

$$S_{\omega\omega}(\Omega) = \frac{\Omega_{\mathrm{m}}^2\phi_0^2}{4\mathrm{ENBW}}\frac{S_{\mathrm{UU}}(\Omega)}{\mathcal{Y}S_{\mathrm{UU}}(\Omega_{\mathrm{mod}})}. \tag{S46}$$

Panel **b** shows the power dependence of $S_{\omega\omega}$ originating form the mechanical displacement noise for four selected microwave powers (2.7 fW, 3.4 fW, 4.3 fW, and 5.4 fW). The most prominent feature in this diagram is the evolution of the noise background, the imprecision noise, which scales as expected inversely with the probe power. To further analyse these data sets, we fit the data with the line-shape given by Eq. (S16) (including a scaling factor) and determine the integrated frequency fluctuations using Eq. (S18). The result is plotted in Fig. S7**c** showing a constant response. This already indicates, that we do not observe strong heating effects due to our blue sideband probing configuration.

In addition to the power dependence, we also study the temperature dependence of the mechanical displacement noise. The data is presented in Fig. S8. Panel **a** shows the temperature dependence of the microwave resonator calibration factor $\mathcal{Y}$. We observe an increase of $\mathcal{Y}$ up to 185 mK followed by a decrease. The increase in $\mathcal{Y}$ originates from an increase in the quality factor of the microwave resonator, which can potentially be attributed to a saturation of two-level fluctuators due to the increased temperature. Above 185 mK, the calibration factor $\mathcal{Y}$ reduces as the quality

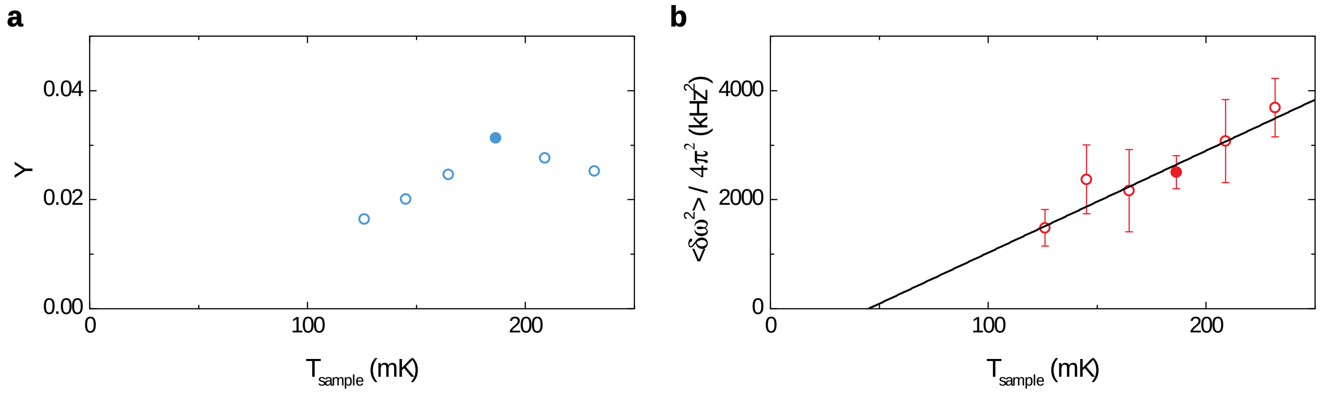


FIG. S8. **Electromechanical coupling rate.** Panel **a** shows the calibration factor $\mathcal{Y}$ as function of the temperature. At 186 mK, the microwave resonator linewidth shows a local minimum resulting in a maximum of $\mathcal{Y}$ (bold dot). Panel **b** displays the integrated area of the mechanical signature $\langle\delta\omega^2\rangle = S_{\omega\omega}(\Omega_\mathrm{m})\Gamma_\mathrm{m}/2$ being proportional to the phonon number as function of temperature. The data discussed in Fig. S7 ($T = 186$ mK) is represented by the solid point. We find a linear dependence of $\langle\delta\omega^2\rangle$ and hence a linear increase of the thermal phonon population as function of temperature. From the slope of the linear fit (black solid line), we derive the vacuum coupling strength. For details, see text.

factor of the microwave resonator decreases. We speculate that this lowering originates either from the generation of quasi-particles (in the aluminium oxide layer) creating an additional loss channel or from the population of thermal photons in the microwave resonator. We repeat the measurement of the down-converted voltage noise spectral density as function of the microwave power along the lines as presented in Fig. S7. However, now we measure as a function of the cryostat temperature and thus obtain the integrated microwave resonator frequency fluctuations $\langle\delta\omega^2\rangle$ as function of temperature. Figure S8**b** shows the temperature dependence of $\langle\delta\omega^2\rangle$. We observe a linear increase in $\langle\delta\omega^2\rangle$ with increasing temperature, which is expected since $\langle\delta\omega^2\rangle$ is proportional to the thermal phonon number. This thermal occupation number increases linear with temperature as for our parameters $k_\mathrm{B}T_\mathrm{sample} \gg \hbar\Omega_\mathrm{m}$. In addition, we also note the data shows a finite offset for $T = 0$, which was interpreted as a back-action temperature by Regal et al. S29. The analysis of the slope in $\langle\delta\omega^2\rangle$ is a second approach to quantify $g_0$. In detail, we fit the data to a linear relation (black solid line) of the form

$$\langle\delta\omega^2\rangle/(2\pi)^2 = s(T_\mathrm{sample})\, T_\mathrm{sample} + c_{\langle\delta\omega^2\rangle}. \tag{S47}$$

We find for the parameters $s(T_\mathrm{sample}) = (1.87 \pm 0.26) \times 10^{10}\,\mathrm{Hz}^2$ and $c_{\langle\delta\omega^2\rangle} = (-8.4 \pm 4.5) \times 10^8\,\mathrm{Hz}^2$. Relating the slope $s(T_\mathrm{sample})$ to the added thermal phonons, i.e. $\bar{n}_\mathrm{m} = k_\mathrm{B}/(\hbar\Omega_\mathrm{m})(T_\mathrm{sample} + T_0)$ [S29], we determine the vacuum coupling strength

$$\frac{g_0^\mathrm{meas}}{2\pi} = \sqrt{\frac{s(T_\mathrm{sample})\hbar\Omega_\mathrm{m}}{2k_\mathrm{B}}} = (1.69 \pm 0.12)\,\mathrm{kHz}. \tag{S48}$$

Note, that the error bars reflect the statistical measurement error. We determine the weighted mean $s(T_\mathrm{sample})$ by fitting the data with an instrumental weight of the statistical deviations in $\langle\delta\omega^2\rangle$. By this we find a standard deviation of $\Delta s(T_\mathrm{sample}) = 0.26 \times 10^{10}\,\mathrm{Hz}^2$. Then the uncertainty in $g_0$ is derived by the statistical propagation of the uncertainty.

Previously we have derived the vacuum coupling strength using Eq. (S27), cf. Fig. S6. This method was derived for optomechanical systems at room temperature [S26]. Using the approach set by Eqs. (S47) and (S48), developed for electromechanical systems at cryogenic temperatures [S29], allows to take a finite temperature offset into account. We reveal an offset temperature of $T_0 = (-45 \pm 30)$ mK in our experiment, cf. Fig. S8**b** and correctly model the increase in frequency fluctuation $\langle\delta\omega^2\rangle(T_\mathrm{sample})$. The optomechanical model derives a lower coupling as it predicts a linear dependence through the origin.

The imprecision noise recorded in the form of the microwave resonator frequency fluctuation power spectral density $S_{\omega\omega}^\mathrm{imp}$ (cf. also Fig. S7) can be used to estimate a flux noise subjected to the SQUID and hereby allows to judge the noise performance of the SQUID. To this end, we transform $S_{\omega\omega}^\mathrm{imp}$ to the power spectral density of the flux noise via

$$S_{\Phi\Phi} = \frac{S_{\omega\omega}}{|(\partial\omega)/(\partial\Phi)|^2}. \tag{S49}$$

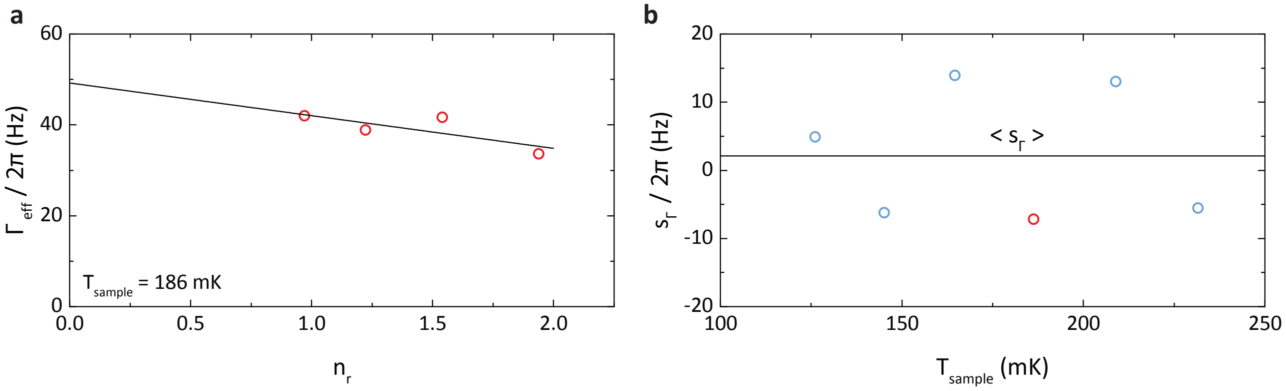


FIG. S9. **Influence of the radiation pressure on the mechanical linewidth.** In panel **a** the linewidth depending on the blue detuned drive tone power in resonator photons is displayed. We find a decrease with power, a potential indication of induced heating. In panel **b** we compare this result (red) to the other sample temperatures (blue). We find fluctuations between $\pm 15\,\mathrm{Hz}$. The average value of $+2\,\mathrm{Hz}$ indicates that the measurement precision is not suffering from induced mechanical phonons given the applied power, as this leads to negative values.

Using the experimentally determined value $S^{\mathrm{imp}}_{\omega\omega}/4\pi^2 = 127\,\mathrm{kHz}^2/\mathrm{Hz}$ for $\bar{n}_\mathrm{r} = 1.6$ in Fig.S7**b** and a responsivity of $\partial(\omega_\mathrm{c}/2\pi)/\partial\Phi = 6.6\,\mathrm{GHz}/\Phi_0$, we find a flux noise density of $1.7\,\mu\Phi_0/\mathrm{Hz}^{1/2}$. This is of the typical order found in undriven Josephson parametric amplifiers, which can be reduced by almost two orders of magnitude using a parametric drive [S30]. Note, that this interprets the entire imprecision noise as flux noise, which might overestimate this value drastically.

## V. HEATING THE MECHANICAL MODE IN BLUE SIDEBAND CONFIGURATION

The determination of the electromechanical coupling constant by measuring the thermal displacement spectrum relies on the equipartition theorem. Thus, we assume that the motion of the string is in thermal equilibrium with the environment, i.e. the temperature of the sample stage of the dilution refrigerator. For our experiment, we use a blue sideband configuration for the readout of the mechanical displacement noise due to the improved sensitivity.[S14] However, this configuration is also known for the amplification and excitation of the displacement on the string [S31–S33]. Besides the probe power independent behavior of $\langle \delta\omega^2 \rangle$ presented in Fig. S7**c**, we present in this section additional experimental data supporting the finding that we are only minimally effected by heating. As a reminder, we set the measurement tone for this experiment to the blue sideband configuration ($\omega_\mathrm{p} = \omega_\mathrm{c} + \Omega_\mathrm{m}$ or $\Delta = \omega_\mathrm{p} - \omega_\mathrm{c} = +\Omega_\mathrm{m}$). Under these conditions, the Stokes (and anti-Stokes) rates $A^+$ ($A^-$) significantly differ due to the filter function of the microwave resonator and the Stokes (anti-Stokes) process becomes highly preferred.[S14] This scattering process also increases (decreases) the mechanical occupation and manifests itself in a modification of the observed mechanical linewidth $\Gamma_\mathrm{eff}$, which consists of the intrinsic linewidth $\Gamma_\mathrm{m}$ and the so-called opto- or electromechanical damping rate $\Gamma_\mathrm{em}$.[S14] For our experiment ($\Delta = +\Omega_\mathrm{m}$), $\Gamma_\mathrm{em}$ is given by

$$\Gamma_\mathrm{em} = -\frac{4\bar{n}_\mathrm{r} g_0^2}{\kappa}. \tag{S50}$$

By introducing the cooperativity $C = 4\bar{n}_\mathrm{r} g_0^2/(\kappa\Gamma_\mathrm{m})$, we can express $\Gamma_\mathrm{eff} = \Gamma_\mathrm{m} + \Gamma_\mathrm{em} = \Gamma_\mathrm{m}(1 + C)$.

Figure S9 shows the change in $\Gamma_\mathrm{eff}$ as function of the probe tone power at a frequency $\omega_\mathrm{p} = \omega_\mathrm{c} + \Omega_\mathrm{m}$ converted to the microwave resonator photon number and as a function of the temperature. Panel **a** shows the measured $\Gamma_\mathrm{eff}$ for a sample temperature of $185\,\mathrm{mK}$. To extract the impact of electromechanical cooling, we fit the data with

$$\Gamma_\mathrm{eff} = s_\Gamma \bar{n}_\mathrm{r} + \Gamma_\mathrm{m} \tag{S51}$$

and obtain $s_\Gamma/2\pi = -(7.2 \pm 4.0)\,\mathrm{Hz}$ and $\Gamma_\mathrm{m}/2\pi = (49 \pm 6)\,\mathrm{Hz}$. Thus, we find only a minimal impact of the electromechanical damping to the measured experimental linewidth $\Gamma_\mathrm{eff}$. Panel **b** shows $s_\Gamma/2\pi$ as a function of the temperature. Here, we find no systematic behavior indicating, that the electromechanical cooling is not dominating $\Gamma_\mathrm{eff}$ in the probe power range used in our $g_0$-experiments and therefore we can neglect heating effects due to the blue sideband configuration in our experiments presented in Sec. IV B. Given the applied photon numbers and the measured vacuum

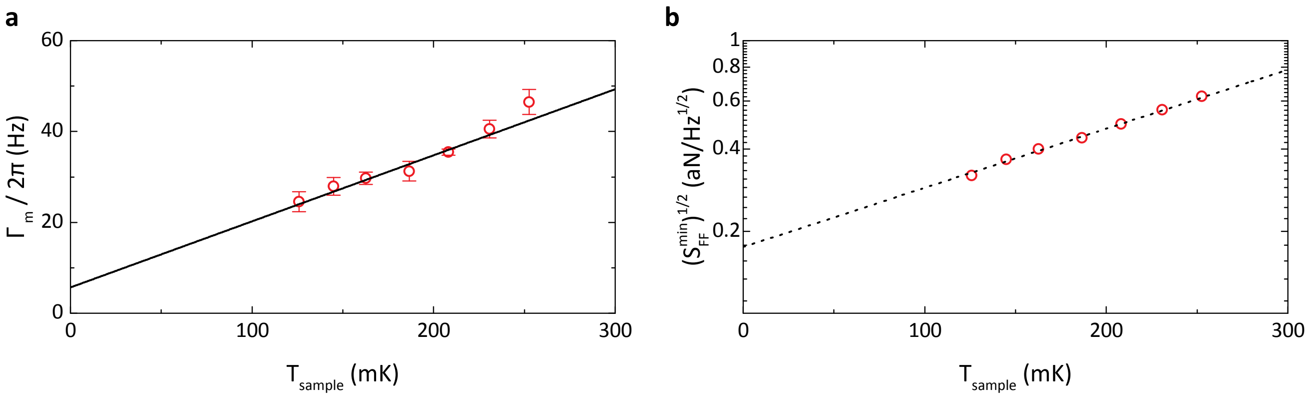


FIG. S10. **Mechanical linewidth and force sensitivity.** Panel **a** shows the mechanical linewidth of the nanostring as a function of the sample temperature. We find a linear increase of $\Gamma_\mathrm{m}$ with temperature (black solid line). Panel **b** shows the minimal force spectral density as function of temperature using Eq. (S53). Note that the mass of the string as well as the damping rate $\Gamma_\mathrm{m}$ depicted in panel **a** affect this value. If not shown, the error bars are smaller than the marker size.

coupling, we estimate an increased phonon occupation by about 4%, which is below the statistical measurement precision of the vacuum coupling strength found to be around 10%. Nevertheless, when we account for this increase in the phonon occupation, we find a corrected electromechanical coupling rate of $g_0/2\pi = (1.62 \pm 0.12)\,\mathrm{kHz}$, that we state in the main text.

## VI. FORCE SENSITIVITY

The noise spectra depicted in Fig. S7 also allows us to quantify the force sensitivity from the displacement noise using [S34]

$$S_\mathrm{FF}^\mathrm{det} = \frac{2S_\mathrm{xx}^\mathrm{det}}{|\chi(\Omega)|^2}, \tag{S52}$$

where $\chi = 1/m_\mathrm{eff}(\Omega^2 - \Omega_\mathrm{m}^2 - i\Gamma_\mathrm{m}\Omega)$ is the mechanical susceptibility of the nanostring. Hereby, we can calculate the spectral force sensitivity presented in Fig. 3**c** of the main text.

Naturally, the force sensitivity is optimal for frequencies equal to the resonance frequency of the mechanical element. Here, the theoretical limit is

$$S_\mathrm{FF}^\mathrm{min} = 4k_\mathrm{B}Tm_\mathrm{eff}\Gamma_\mathrm{m}. \tag{S53}$$

Figure S10**b** shows the best force sensitivity as a function of the sample temperature. For increasing temperature, we find an increase in $S_\mathrm{FF}$ due to the impact of the enlarged mechanical linewidth.

## VII. SCALING OF THE ELECTROMECHANICAL COUPLING

Due to the nature of the inductive coupling, the electromechanical coupling rate is flux tunable (see. Eq. (1) in the main text). Thus, we expect a linear scaling of the electromechanical coupling rate with $\partial\omega_\mathrm{c}/\partial\Phi$ and $B_\mathrm{ext}$. As discussed in the main text, one option to explore the scaling of $g_0$ are thermal displacement noise experiments. Alternatively, and more time efficiently, on can measure the frequency shift of the microwave resonator for a fixed mechanical excitation amplitude. In this experiment, the signal amplitudes are significantly larger resulting in a faster data acquisition. In detail, we use a piezo actuator mounted on the outside of the sample enclosure to excite the nanostring. For a fixed excitation voltage applied to the piezo actuator, we then record the displacement induced frequency shift of the microwave resonator $\delta\omega_\mathrm{c}$ for various $\partial\omega_\mathrm{c}/\partial\Phi$ and $B_\mathrm{ext}$.

For this measurement we employ the setup depicted in Fig. S1**a** and **b**. The temperature is set to $T_\mathrm{sample} \approx 120\,\mathrm{mK}$. We start with the investigation of the scaling with $\partial\omega_\mathrm{c}/\partial\Phi$ and keep a constant value of $B_\mathrm{ext} \approx -440\,\mu\mathrm{T}$. Note that we slightly modify $B_\mathrm{ext}$ by up to $20\,\mu\mathrm{T}$ in order to tune to the bias points with desired $\partial\omega_\mathrm{c}/\partial\Phi$. However, as this represents only a minimal modification of the total $B_\mathrm{ext}$, we assume the static bias field as fixed for our analysis.

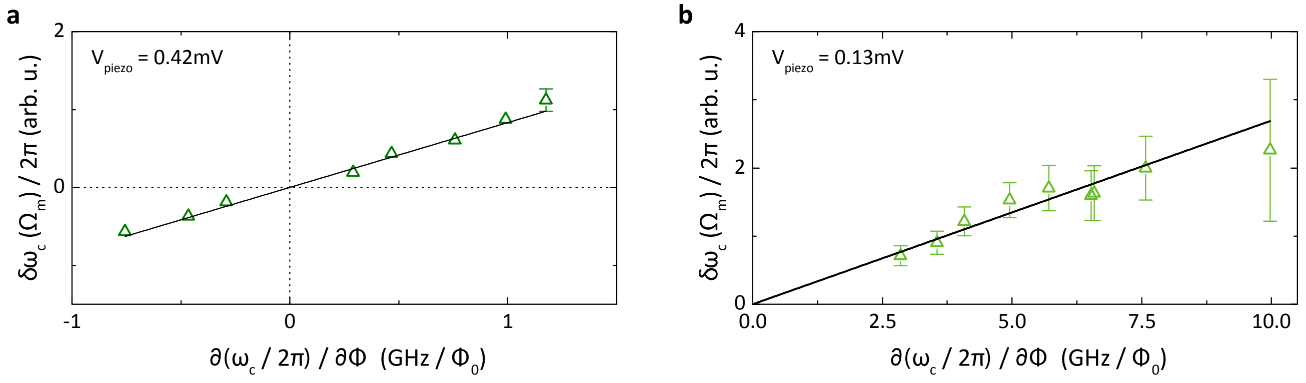


FIG. S11. **Driven frequency shift.** Panel **a** shows the extracted frequency shift $\delta\omega_c(\Omega_m)$ from Fig. 4**a** in the main text over the resonator responsivity $\partial\omega_c/\partial\Phi$. In case of negative responsivity we multiplied the coupling strength by $-1$ to show the linear dependence beyond the sweet spot. The expected linear tuning is confirmed. In panel **b**, we summarize the frequency shift for higher responsivities, where we have reduced probe tone power and piezo drive voltage. By this we confirm the linearity for responsivitites up to $10\,\mathrm{GHz}/\Phi_0$. The reduced drive voltage leads to a decreased proportionality as less phonons are excited by the piezo actuator. If not shown, the error bars are smaller than the marker size.

We measure $\delta\omega_c$, by applying a constant microwave tone with frequency $\omega = \omega_c$ ($\Delta = 0$) to the sample. The signal from the sample is then down-converted using an LO frequency of $\omega_{LO} = \omega$. We use the vector network analyser to excite the piezo actuator and thus provide an oscillating force to our mechanically compliant nanostring. On resonance, a mechanical displacement is excited and thus the microwave resonator frequency shifts according to the electromechanical Hamiltonian. This frequency shift manifests itself in the down-converted signal, which we record with the vector network analyser. In detail, the measured scattering parameter of the vector network analyser is therefore proportional to the frequency shift $\delta\omega_c$. In analogy to Ref. S17 we define

$$P_{\mathrm{hom}} \propto \frac{2K_\Psi}{\Omega^2}\left(\delta\omega_c\right)^2 . \tag{S54}$$

Here, the function $K_\Psi = \tilde{K}^{x,U}(\Omega_m, \Delta = 0)$ contains the parameters of the microwave resonator and relates them to the resonance frequency of the nanostring, cf. Eq. (S19). The input parameters $\eta$ and $\kappa$ entering $K_\Psi$ are determined prior to each experiment by measuring the microwave transmission of the microwave resonator. In this way, we obtain a quantity proportional to the frequency shift $\delta\omega_c$ from the frequency dependent measurement of $P_{\mathrm{hom}}$. The corresponding data is presented in Fig. 4a in the main text as frequency shift $\delta\omega_c$ derived from Eq. (S54) and the recorded $P_{\mathrm{hom}}$. We fit a Lorentzian lineshape to the data and plot the amplitude of the Lorenzian at $\Omega_m$ for two different piezo drive amplitudes in Fig. S11. We assume, that the fixed mechanical excitation force stimulates a fixed mechanical amplitude response independent of the particular $\partial\omega_c/\partial\Phi$ chosen. Then, the recorded $\delta\omega_c(\Omega_m)$ is proportional to $g_0$ and hence we can rescale these datasets to complete the scaled data presented in Fig. 4 b and c in the main text.

Figure S11**a** and **b** show the dependence of $\delta\omega_c(\Omega_m)$ as a function of $\partial\omega_c/\partial\Phi$. For both panels, we observe a linear dependence. As our measurement scheme is restricted to the linear transduction of the mechanical amplitude to a frequency shift, we investigate two mechanical excitation regimes: (i) we excite larger mechanical amplitudes using a piezo actuator voltage of $V_{\mathrm{piezo}} = 0.42\,\mathrm{mV}$ for testing the smaller coupling strengths of up to 0.5 kHz. (ii) For larger coupling rates, we reduce the mechanical amplitde by setting the piezo actuator voltage to $V_{\mathrm{piezo}} = 0.13\,\mathrm{mV}$. Note that the chosen piezo actuator voltages are still in the linear mechanical response regime. This is confirmed by the observation that the relative slopes of $0.97 \times \partial\omega_c/\partial\Phi$ for $V_{\mathrm{piezo}} = 0.42\,\mathrm{mV}$ and $0.27 \times \partial\omega_c/\partial\Phi$ for $V_{\mathrm{piezo}} = 0.13\,\mathrm{mV}$ compare well to the ratio of their excitation voltages.

As already indicated above, we relate the results of Fig. S11 to the electromechanical coupling rate measured via the thermal displacement spectra of the nanostring.

Considering this combined dataset, which is presented in Fig. 4 of the main text, we extract the scaling of the electromechanical vacuum coupling strength with $B_{\mathrm{ext}}$ to 3.13 MHz/T. Here, we set $\partial(\omega_c/2\pi)/\partial\Phi = 6.6\,\mathrm{GHz}/\Phi_0$. This corresponds to $g_0 = 1.38\,\mathrm{kHz}$ at the investigated magnetic field bias of $B_{\mathrm{ext}} = -440\,\mu\mathrm{T}$, indicated by the red cross in Fig. 4**b** in the main text. In analogy to the procedure detailed above, we complement the scaled data obtained by measuring the thermal displacement noise with respect to the magnetic field bias $B_{\mathrm{ext}}$ resulting in Fig. 4**c** of the main text.

## VIII. STRONGLY MECHANICALLY DRIVEN ELECTROMECHANICS

Next, we discuss the spectral features of the microwave resonator's transfer function, when the mechanical motion is excited to a high amplitude state. Here, we we describe the amplitude of the displacement of the driven mechanical motion of a nanostring by

$$x(t) = x_0 \sin\left(\Omega_\mathrm{m} t\right). \tag{S55}$$

The field amplitude of the electromechanical microwave resonator $a(t)$ is given by [S26]

$$\partial_\mathrm{t} a(t) + \left[\frac{\kappa}{2} + i\left(-\omega_\mathrm{c} + Gx(t)\right)\right] a(t) = \sqrt{\eta_\mathrm{c}\kappa}\, s_\mathrm{in}(t). \tag{S56}$$

Here, we relate the external to total linewidth via $\eta_\mathrm{c} = \kappa_\mathrm{ext}/\kappa$. The incoming probe signal is given by $s(t) = s_\mathrm{in}\exp(i\omega_\mathrm{p} t)$. The solution of the differential equation is solved by a homogeneous and particular solution $a(t) = a_\mathrm{h}(t) + a_\mathrm{p}(t)$. The homogeneous solution for $\partial_\mathrm{t} a_\mathrm{h}(t) + b a_\mathrm{h}(t) = 0$ is [S35, S36]

$$a_\mathrm{h}(t) = A_0 \exp\left[\left(-\frac{\kappa}{2} + i\omega_\mathrm{c}\right) t + i\beta \cos\left(\Omega_\mathrm{m} t\right)\right], \tag{S57}$$

where we have introduced the parameter $\beta = g_0 x_0/(x_\mathrm{zpm}\Omega_\mathrm{m})$. As our measurement's detection bandwidth is on the order of Hz, we can neglect the homogeneous solution $a_\mathrm{h}$ as it is exponentially suppressed with a rate of $\kappa/2$ (being in the MHz range) [S35, S36]. Thus we can describe our experiments sufficiently by $a(t) = a_\mathrm{p}(t)$,[S35, S36]

$$a_\mathrm{p}(t) = \sqrt{\eta_\mathrm{c}\kappa}\, s_\mathrm{in} \sum_{n=-\infty}^{\infty} \frac{(-i)^n J_n(\beta)}{\frac{\kappa}{2} + i(\Delta + n\Omega_\mathrm{m})} \exp\left[i(\omega + n\Omega_\mathrm{m})t + i\beta\cos(\Omega_\mathrm{m} t)\right]. \tag{S58}$$

The detected output field is then $s_\mathrm{out} = s_\mathrm{in} - \sqrt{\eta_\mathrm{c}\kappa}\, a_\mathrm{p}$. In the experiment (cf. Fig. 5 in the main text), we plot the absolute square of the complex transmission function which is given by [S35, S36]

$$|S_{21}|^2 = |\frac{s_\mathrm{out}}{s_\mathrm{in}}|^2 = 1 - \eta_\mathrm{c}\kappa^2(1 + \eta_\mathrm{c}) \sum_{n=-\infty}^{\infty} \frac{J_n^2(\beta)}{\frac{\kappa^2}{4} + (\Delta + n\Omega_\mathrm{m})^2}. \tag{S59}$$

This result is identical to Eq. (2) in the main text, which we quantitatively compare with the data.

## IX. SUMMARY OF THE ELECTROMECHANICAL HYBRID SYSTEM

Table S1 summarises the parameters of the components of the electromechanical system consisting of (i) the mechanical string, (ii) the coplanar waveguide resonator (CPW), (iii) the superconducting quantum interference device (SQUID), and (iv) the flux-tunable microwave resonator (FTR).


[S1] P. Schmidt, D. Schwienbacher, M. Pernpeintner, F. Wulschner, F. Deppe, A. Marx, R. Gross, and H. Huebl, Appl. Phys. Lett. **113**, 152601 (2018).

[S2] M. Göppl, A. Fragner, M. Baur, R. Bianchetti, S. Filipp, J. M. Fink, P. J. Leek, G. Puebla, L. Steffen, and A. Wallraff, J. Appl. Phys. **104**, 113904 (2008).

[S3] D. M. Pozar, Microwave engineering, 4th ed. (John Wiley & Sons, Inc., Hoboken, NJ, 2012).

[S4] M. Wallquist, V. S. Shumeiko, and G. Wendin, Phys. Rev. B **74**, 791 (2006).

[S5] W. Wustmann and V. Shumeiko, Phys. Rev. B **87**, 184501 (2013).

[S6] S. Pogorzalek, K. G. Fedorov, L. Zhong, J. Goetz, F. Wulschner, M. Fischer, P. Eder, E. Xie, K. Inomata, T. Yamamoto, Y. Nakamura, A. Marx, F. Deppe, and R. Gross, Phys. Rev. Appl. **8**, 024012 (2017).

[S7] P. Bhupathi, P. Groszkowski, M. P. DeFeo, M. Ware, F. K. Wilhelm, and B. L. T. Plourde, Phys. Rev. Appl. **5**, 024002 (2016).

[S8] The deviations from the exact model are of the order of 5 %.

[S9] F. E. Terman, Radio Engineers' Handbook, 1st ed. (McGraw-Hill Book Company Inc., New York, 1943).

[S10] M. J. Schwarz, Gradiometric tunable-gap flux qubits in a circuit QED architecture, Ph.D. thesis, Walther-Meißner-Institut and Technische Universität München (2014).

[S11] J. Bourassa, F. Beaudoin, J. M. Gambetta, and A. Blais, Phys. Rev. A **86**, 013814 (2012).

| | Parameter | Value | Comments |
|---|---|---|---|
| **String** | Mechanical eigenfrequency | $\Omega_\mathrm{m}/2\pi = 6.343\,16\,\mathrm{MHz}$ | mode 4 |
| | Mechanical linewidth (FWHM) | $\Gamma_\mathrm{m}/2\pi = 25\,\mathrm{Hz}$ | $T = 110\,\mathrm{mK}$ |
| | Length of the string | $l = 20\,\mu\mathrm{m}$ | |
| | Cross section of the string | $S = w \cdot t = 110 \cdot 200\,\mathrm{nm}^2$ | |
| | Tensile stress of the string | $\sigma = 170\,\mathrm{MPa}$ | $T = 110\,\mathrm{mK}$ |
| | Young's modulus (aluminium) | $E_\mathrm{Y} = 70\,\mathrm{GPa}$ | [S25] |
| **CPW** | Bare cpw eigenfrequency | $\omega_0/2\pi = 9.85\,\mathrm{GHz}$ | |
| | CPW length | $l_\mathrm{c} = 2.930\,\mathrm{mm}$ | |
| | CPW dimensions (width, gap) | $w_\mathrm{c} = 10\,\mu\mathrm{m}$ $s_\mathrm{c} = 8\,\mu\mathrm{m}$ | |
| | CPW resonator inductance, capacitance | $L_\mathrm{c} = 1.17\,\mathrm{nH}$ $C_\mathrm{c} = 224\,\mathrm{fF}$ | |
| | CPW impedance | $Z = 56\,\Omega$ | |
| | Eff. dielectric constant | $\epsilon_\mathrm{eff} = 6.45$ | |
| **SQUID** | SQUID inductances | $L_\mathrm{kin} = 41\,\mathrm{pH}$ $L_\mathrm{geo} = 19\,\mathrm{pH}$ | |
| | Josephson inductance | $L_\mathrm{J} = 0.36\,\mathrm{nH}$ | at sweet spot |
| | Critical current | $I_\mathrm{c} = 442\,\mathrm{nA}$ | single junction |
| | Loop area | $A_\mathrm{loop} = 44.6\,\mu\mathrm{m}^2$ | |
| | Screening parameter | $\beta_\mathrm{L} = 0.013$ | |
| **FTR** | Sweet spot frequency | $\omega_\mathrm{c}/2\pi = 7.445\,\mathrm{GHz}$ | |
| | Sweet spot intrinsic linewidth | $\kappa_\mathrm{int}/2\pi = 2\,\mathrm{MHz}$ | $T = 110\,\mathrm{mK}$ |
| | External microwave coupling | $\kappa_\mathrm{ext}/2\pi = 0.5\,\mathrm{MHz}$ | |

TABLE S1. *Summary of all sample parameters.*


[S12] P. Nation, M. Blencowe, and E. Buks, Phys. Rev. B **78**, 104516 (2008).
[S13] C. Eichler and A. Wallraff, Eur. Phys. J. QT **1** (2014).
[S14] M. Aspelmeyer, T. J. Kippenberg, and F. Marquardt, Rev. Mod. Phys. **86**, 1391 (2014).
[S15] A. Clerk, M. Devoret, S. Girvin, F. Marquardt, and R. Schoelkopf, Rev. Mod. Phys. **82**, 1155 (2010).
[S16] J. S. Huber, G. Rastelli, M. J. Seitner, J. Kölbl, W. Belzig, M. I. Dykman, and E. M. Weig, "Detecting squeezing from the fluctuation spectrum of a driven nanomechanical mode," (2019), arXiv:1903.07601v2.
[S17] M. Pernpeintner, T. Faust, F. Hocke, J. P. Kotthaus, E. M. Weig, H. Huebl, and R. Gross, Appl Phys Lett **105**, 123106 (2014).
[S18] T. S. Biswas, J. Xu, X. Rojas, C. Doolin, A. Suhel, K. S. D. Beach, and J. P. Davis, Nano Lett. **14**, 2541 (2014).
[S19] K. Gajo, S. Schüz, and E. M. Weig, Appl. Phys. Lett. **111**, 133109 (2017).
[S20] M. Pernpeintner, P. Schmidt, D. Schwienbacher, R. Gross, and H. Huebl, Phys. Rev. Appl. **10**, 4448 (2018).
[S21] H. Okamoto, T. Kamada, K. Onomitsu, I. Mahboob, and H. Yamaguchi, Appl. Phys. Express **2**, 062202 (2009).
[S22] F. Hocke, M. Pernpeintner, X. Zhou, A. Schliesser, T. J. Kippenberg, H. Huebl, and R. Gross, Appl. Phys. Lett. **105**, 133102 (2014).
[S23] J. Weaver, S. P. Timoshenko, and D. H. Young, Vibrational problems in engineering (John Wiley & Sons, 1990).
[S24] S. S. Verbridge, J. M. Parpia, R. B. Reichenbach, L. M. Bellan, and H. G. Craighead, J. Appl. Phys. **99**, 124304 (2006).
[S25] J. Sulkko, M. A. Sillanpää, P. Häkkinen, L. Lechner, M. Helle, A. Fefferman, J. Parpia, and P. J. Hakonen, Nano Lett. **10**, 4884 (2010).
[S26] M. L. Gorodetsky, A. Schliesser, G. Anetsberger, S. Deleglise, and T. J. Kippenberg, Optics Express **18**, 23236 (2010).
[S27] In the case of Gorodetsky et al. Ref. S26 the measured quantity were the photo-current fluctuations.
[S28] Note, that this result is independent of the presence of modulation tone as long as the phase modulation frequency is set detuned (non-overlapping) with the mechanical signal. We implicitly assume this condition here.
[S29] C. A. Regal, J. D. Teufel, and K. W. Lehnert, Nat. Phys. **4**, 555 (2008).
[S30] M. Hatridge, R. Vijay, D. H. Slichter, J. Clarke, and I. Siddiqi, Phys. Rev. B **83** (2011).
[S31] F. Hocke, X. Zhou, A. Schliesser, T. J. Kippenberg, H. Huebl, and R. Gross, New J. Phys. **14**, 123037 (2012).
[S32] V. Singh, S. J. Bosman, B. H. Schneider, Y. M. Blanter, A. Castellanos-Gomez, and G. A. Steele, Nat. Nanotechnol. **9**, 820 (2014).
[S33] I. C. Rodrigues, D. Bothner, and G. A. Steele, Nat. Commun. **10**, 5359 (2019).
[S34] J. D. Teufel, T. Donner, M. A. Castellanos-Beltran, J. W. Harlow, and K. W. Lehnert, Nat. Nanotechnol. **4**, 820 (2009).
[S35] A. Schliesser, R. Rivière, G. Anetsberger, O. Arcizet, and T. J. Kippenberg, Nat. Phys. **4**, 415 (2008).
[S36] X. Zhou, F. Hocke, A. Schliesser, A. Marx, H. Huebl, R. Gross, and T. J. Kippenberg, Nat. Phys. **9**, 179 (2013).
